# Supplementary material for: Stabilize, Decompose, and Denoise: Self-Supervised Fluoroscopy Denoising
Source: arXiv:2208.14022 source file (2022-08-30)
Supplement: Supplementary file 1 [file t4.tex]

\begin{figure}
    \centering
        \begin{minipage}[t]{0.19\textwidth}
			\centering
			\includegraphics[width=1\textwidth]{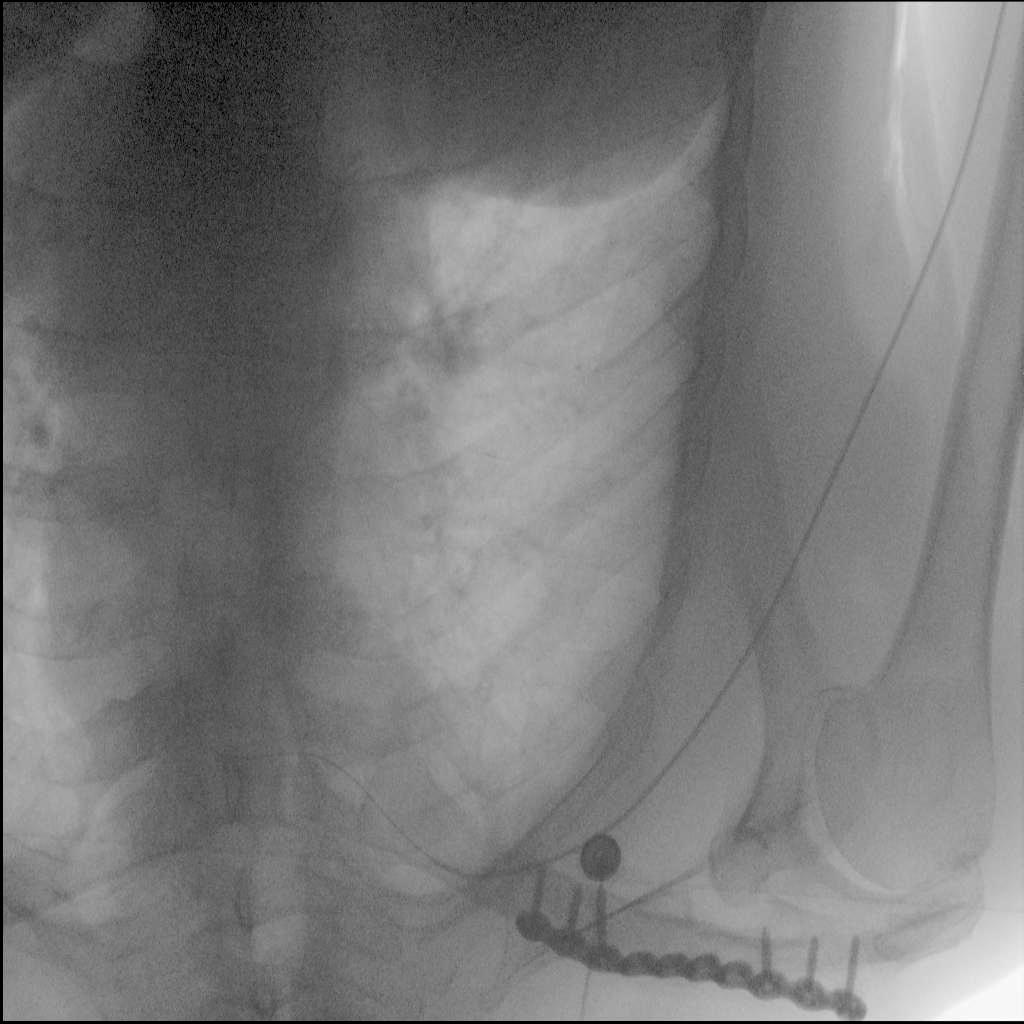}
			\includegraphics[width=1\textwidth]{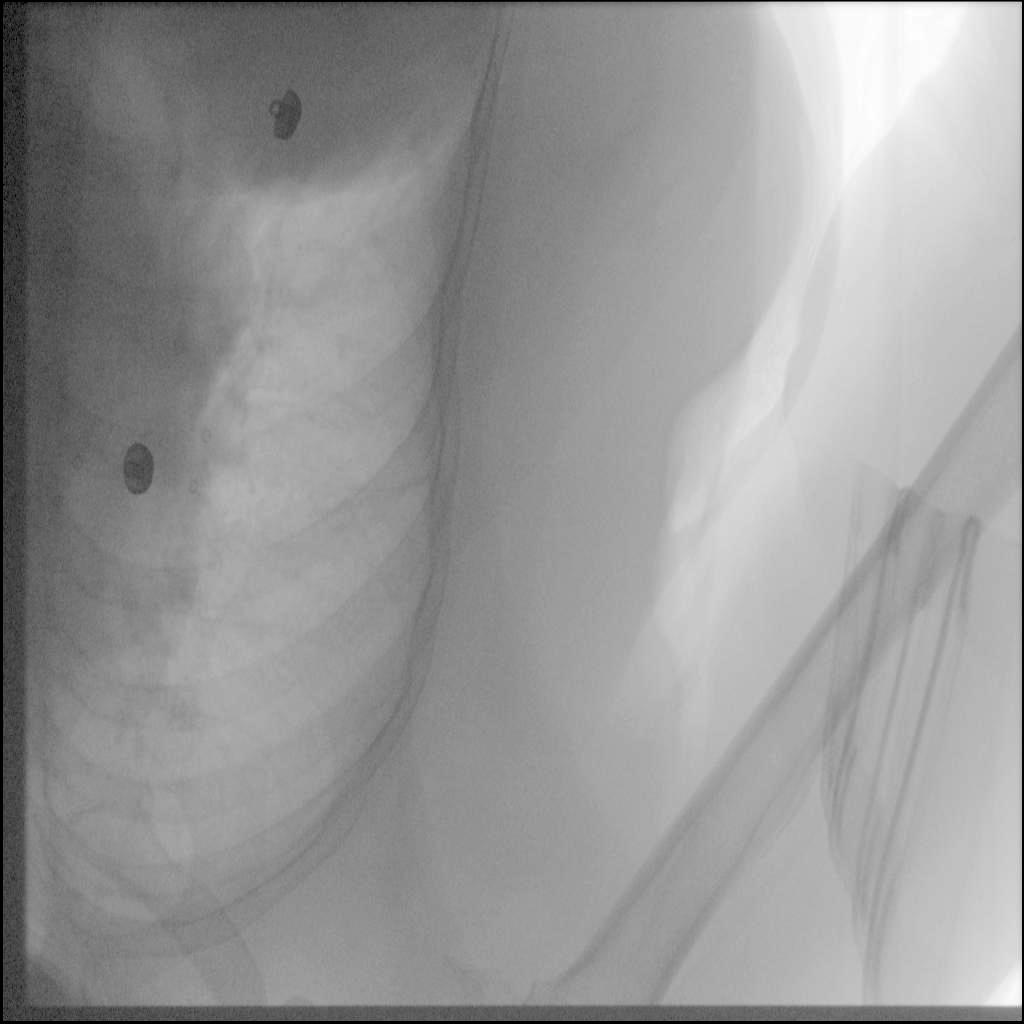}
			\includegraphics[width=1\textwidth]{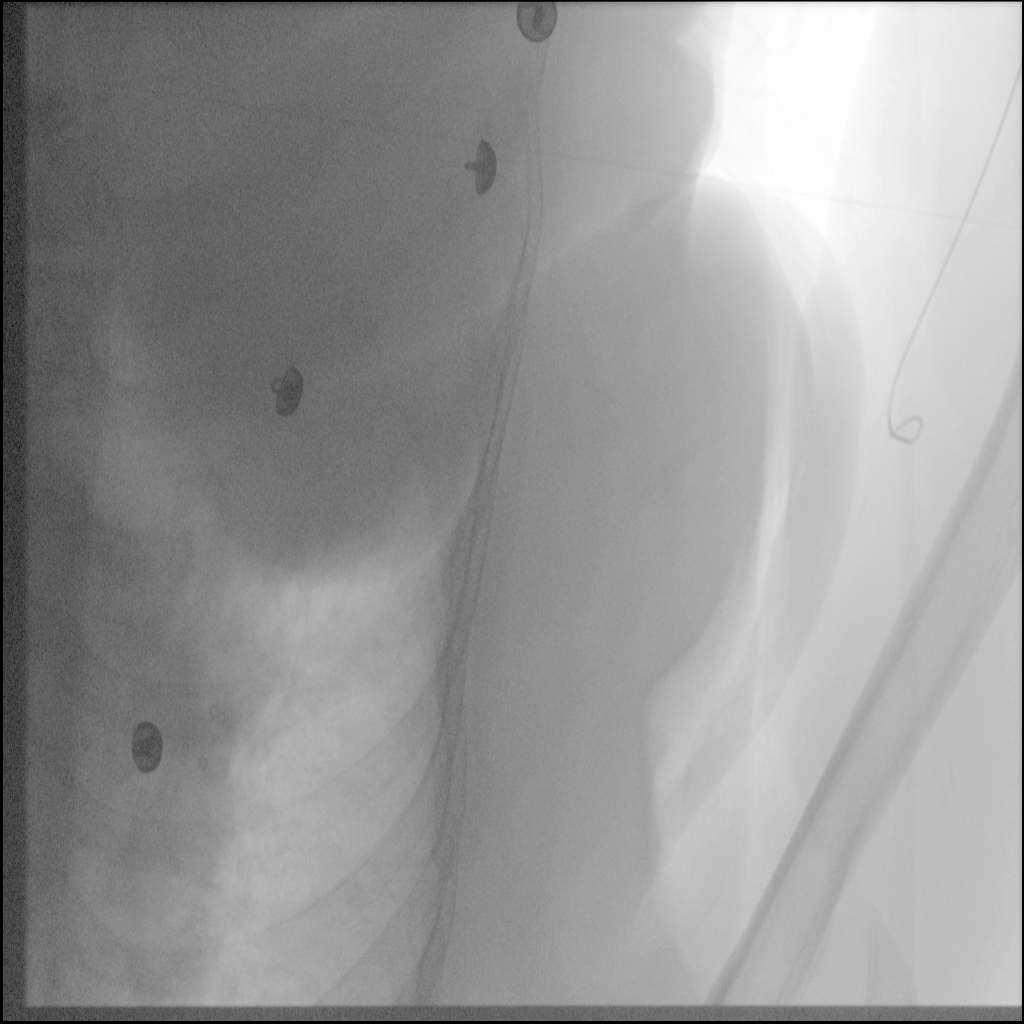}
			\includegraphics[width=1\textwidth]{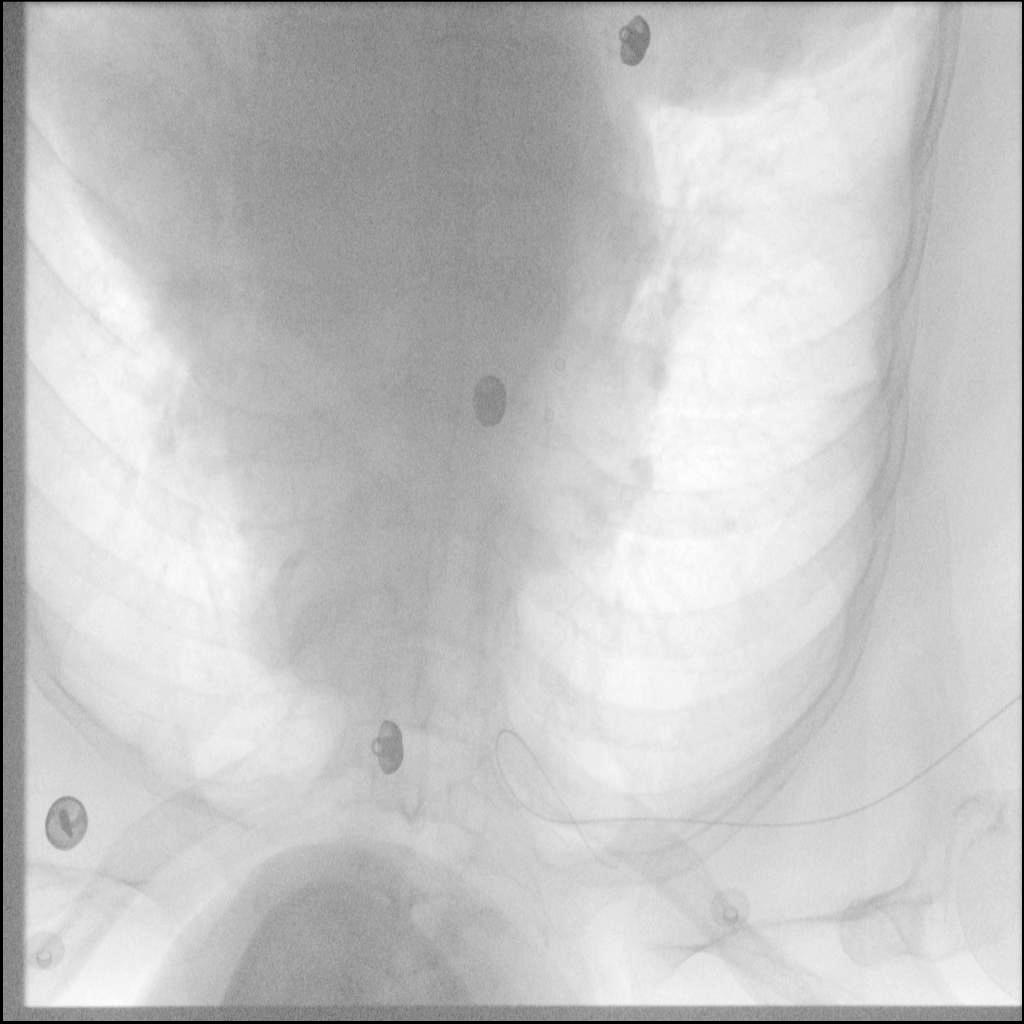}
			\includegraphics[width=1\textwidth]{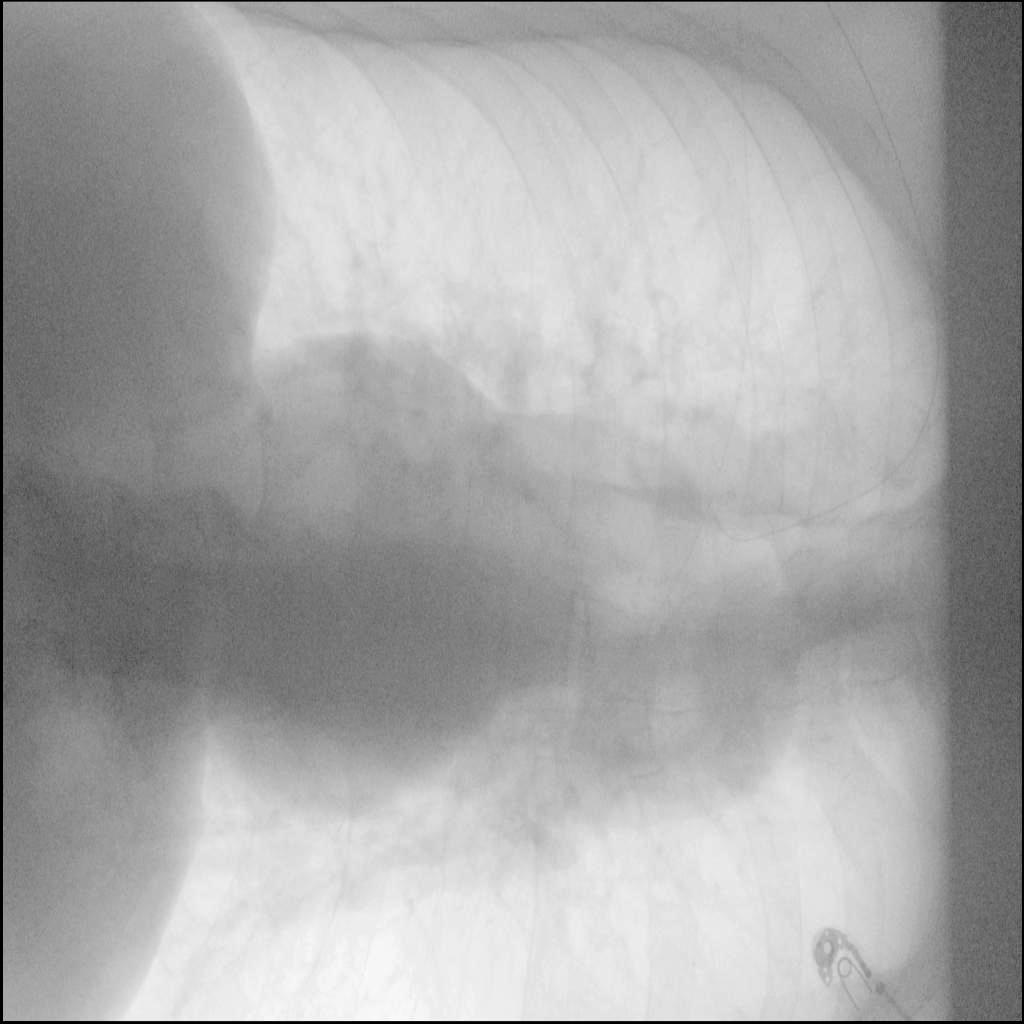}
			\includegraphics[width=1\textwidth]{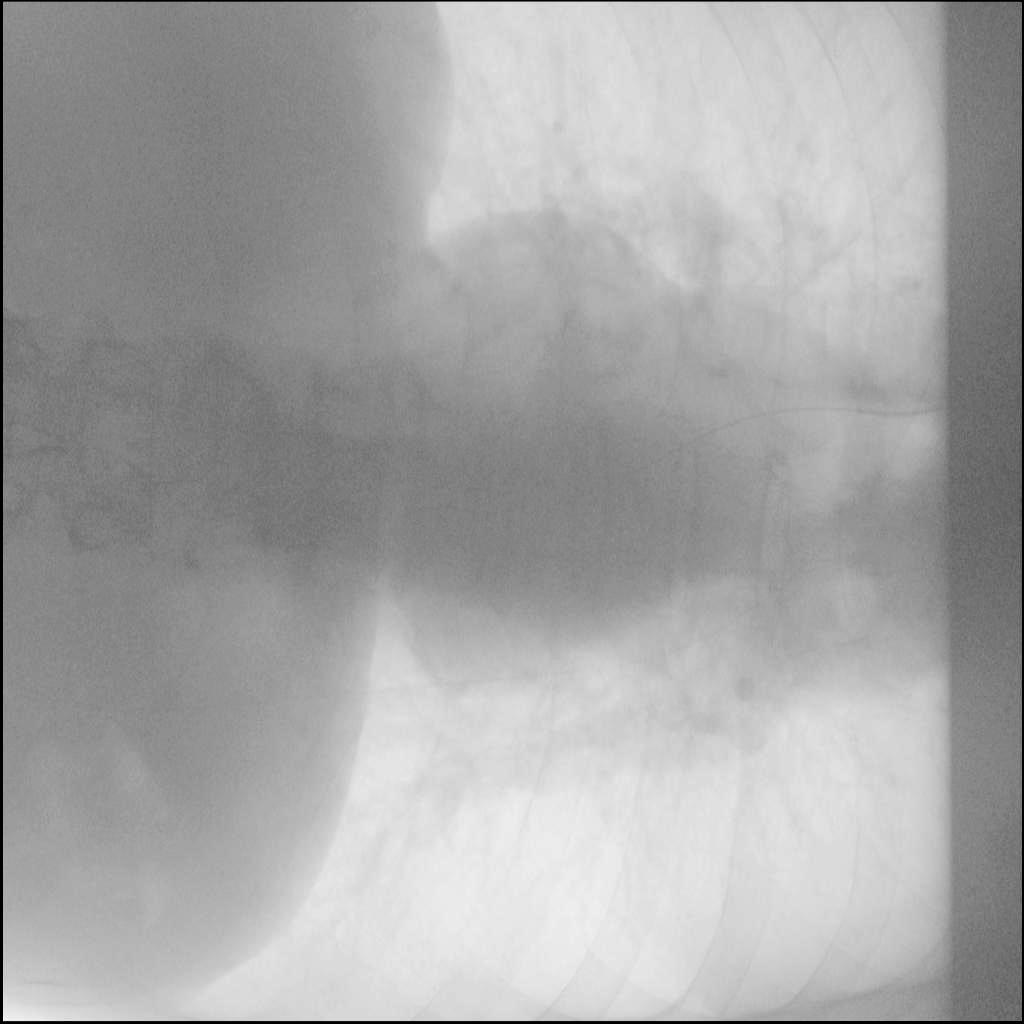}
			\includegraphics[width=1\textwidth]{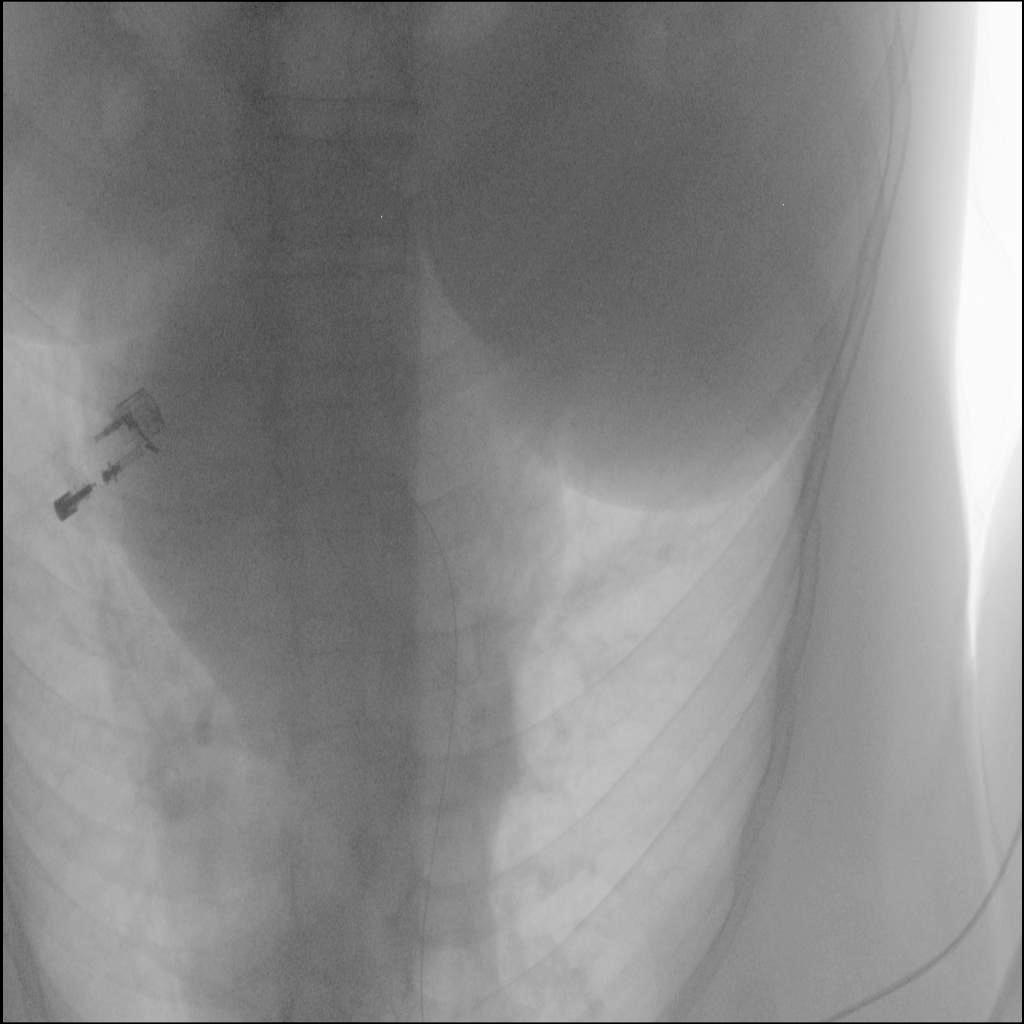}
			\scriptsize{Input}
		\end{minipage}
		\begin{minipage}[t]{0.19\textwidth}
			\centering
			\includegraphics[width=1\textwidth]{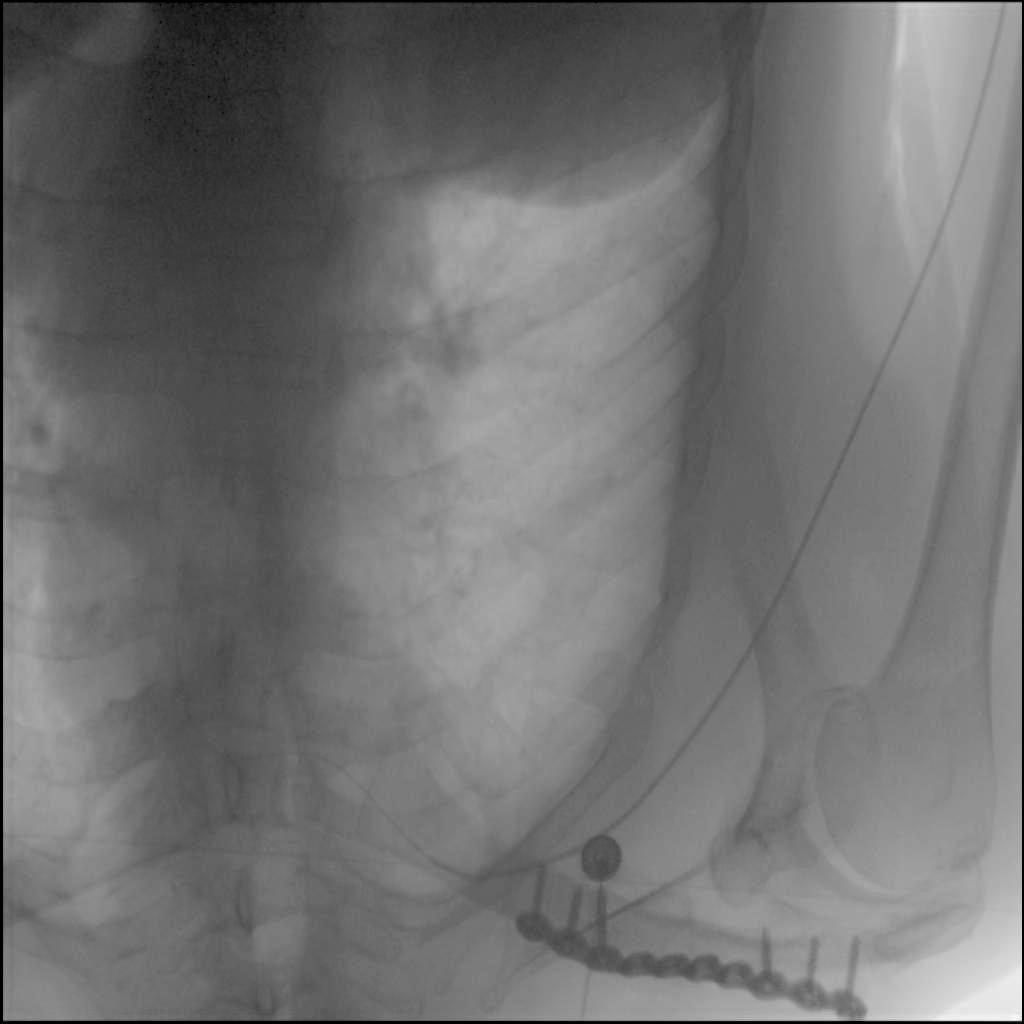}
			\includegraphics[width=1\textwidth]{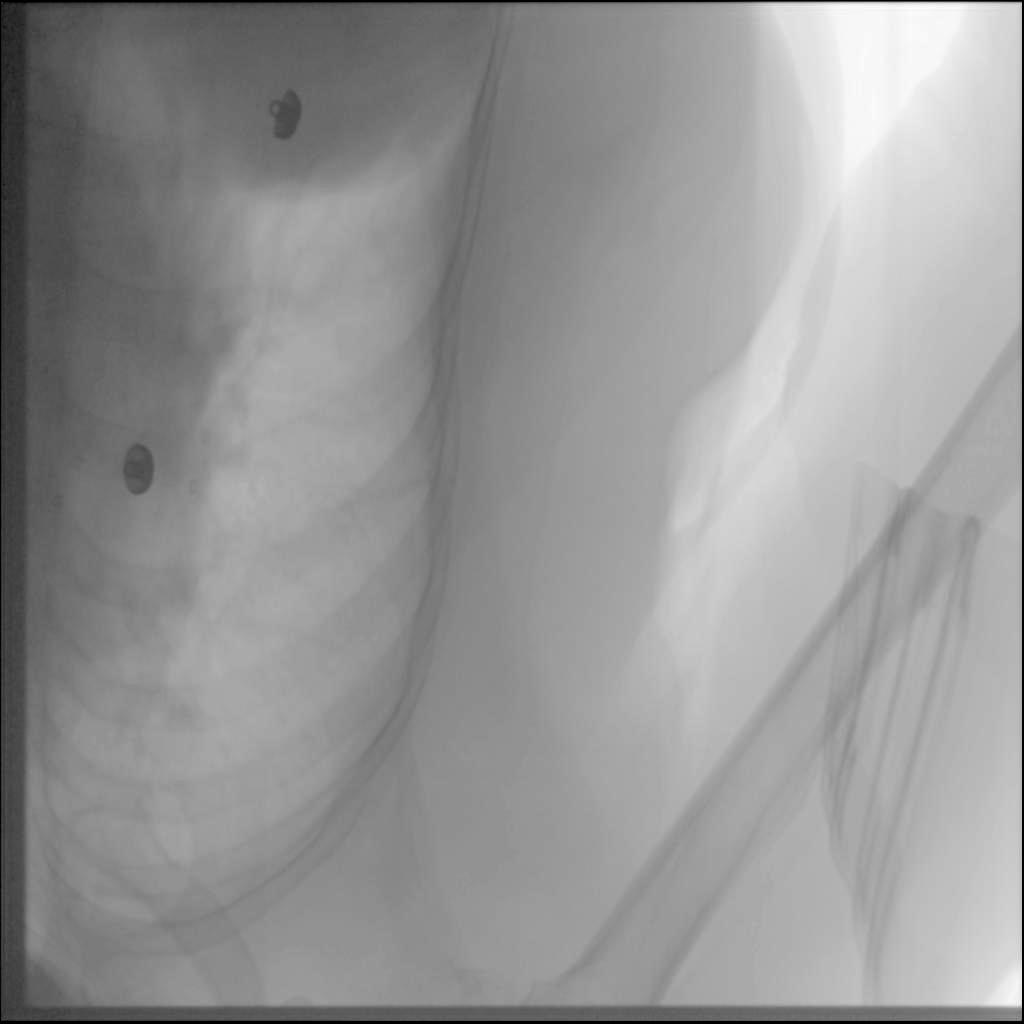}
			\includegraphics[width=1\textwidth]{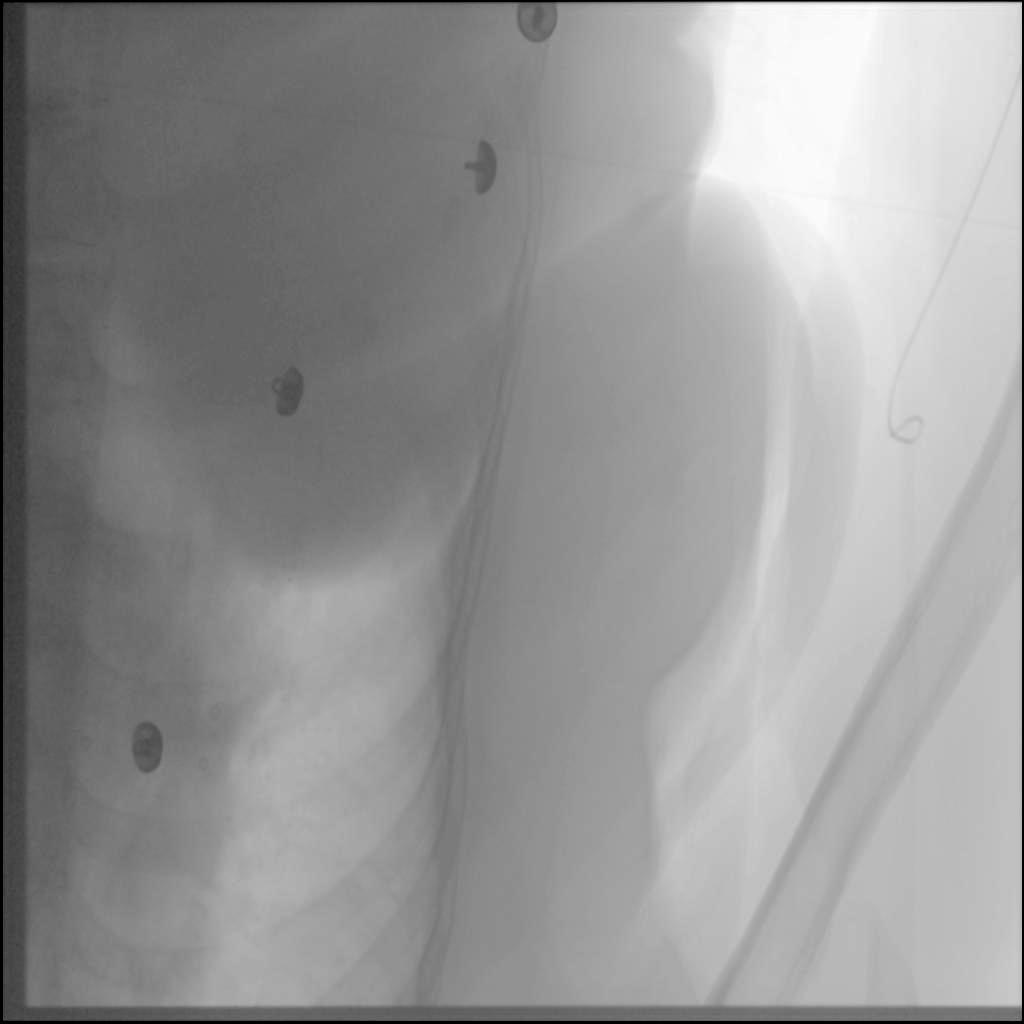}
			\includegraphics[width=1\textwidth]{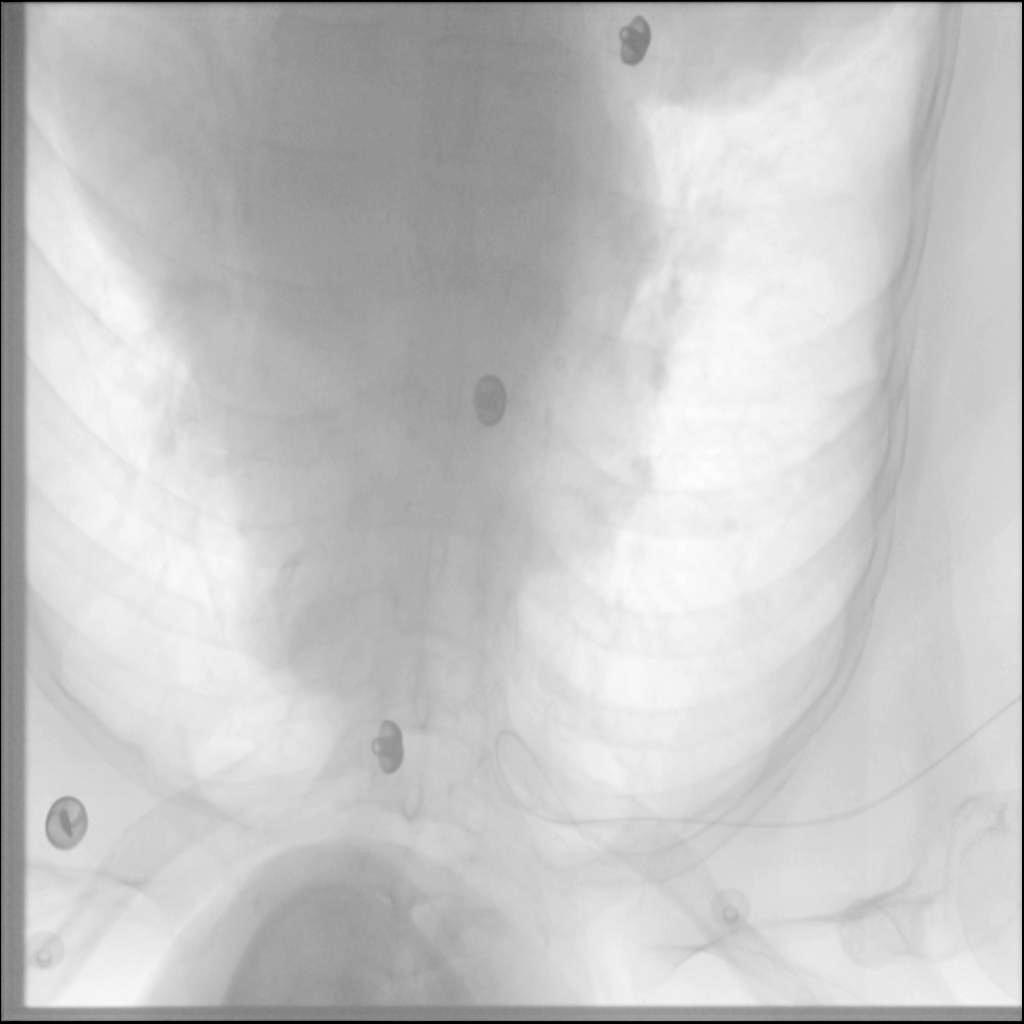}
			\includegraphics[width=1\textwidth]{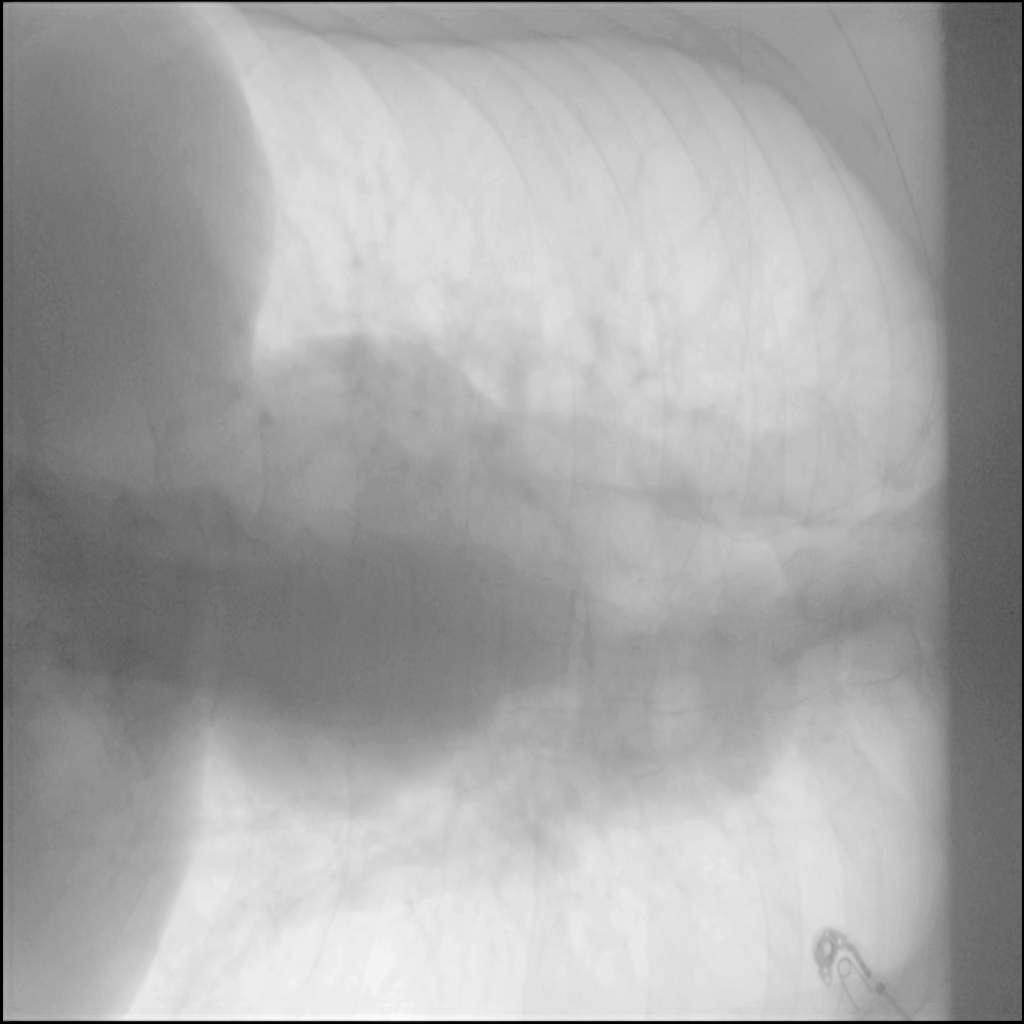}
			\includegraphics[width=1\textwidth]{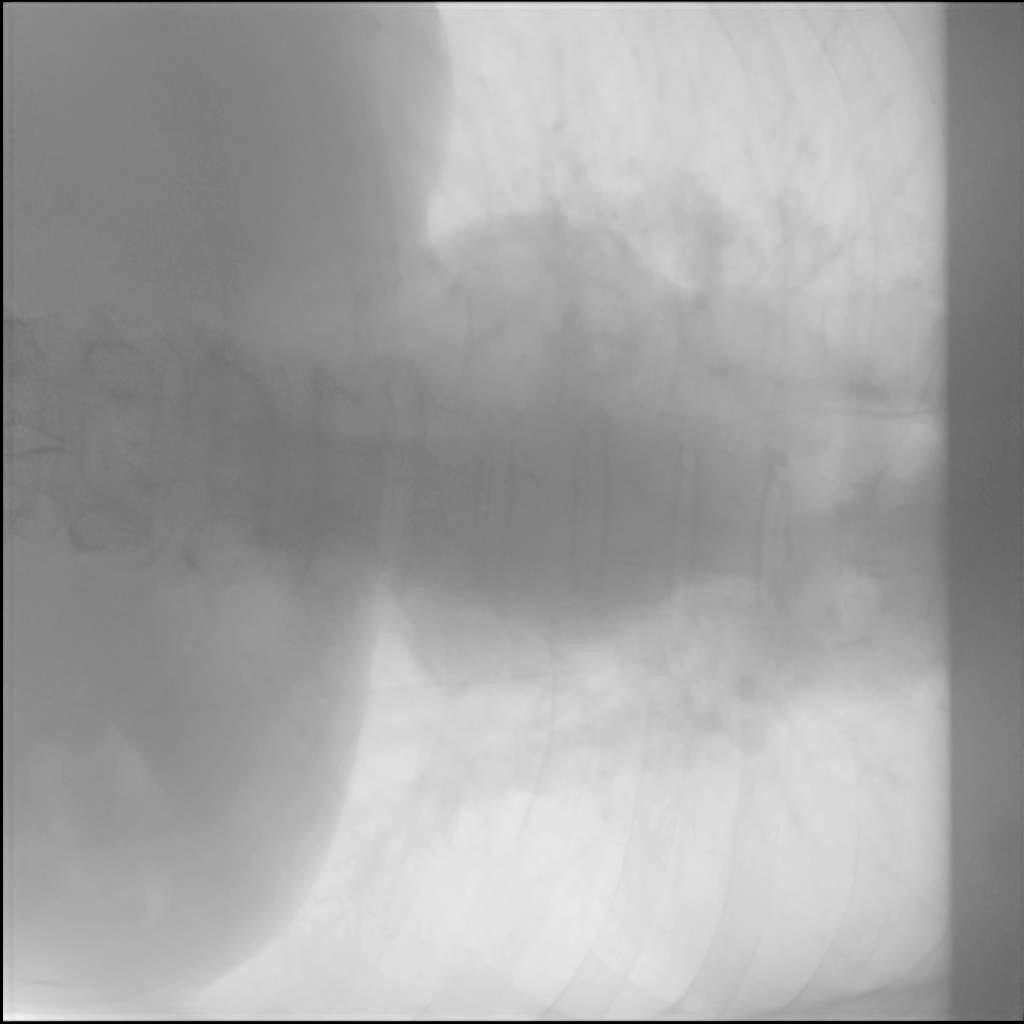}
			\includegraphics[width=1\textwidth]{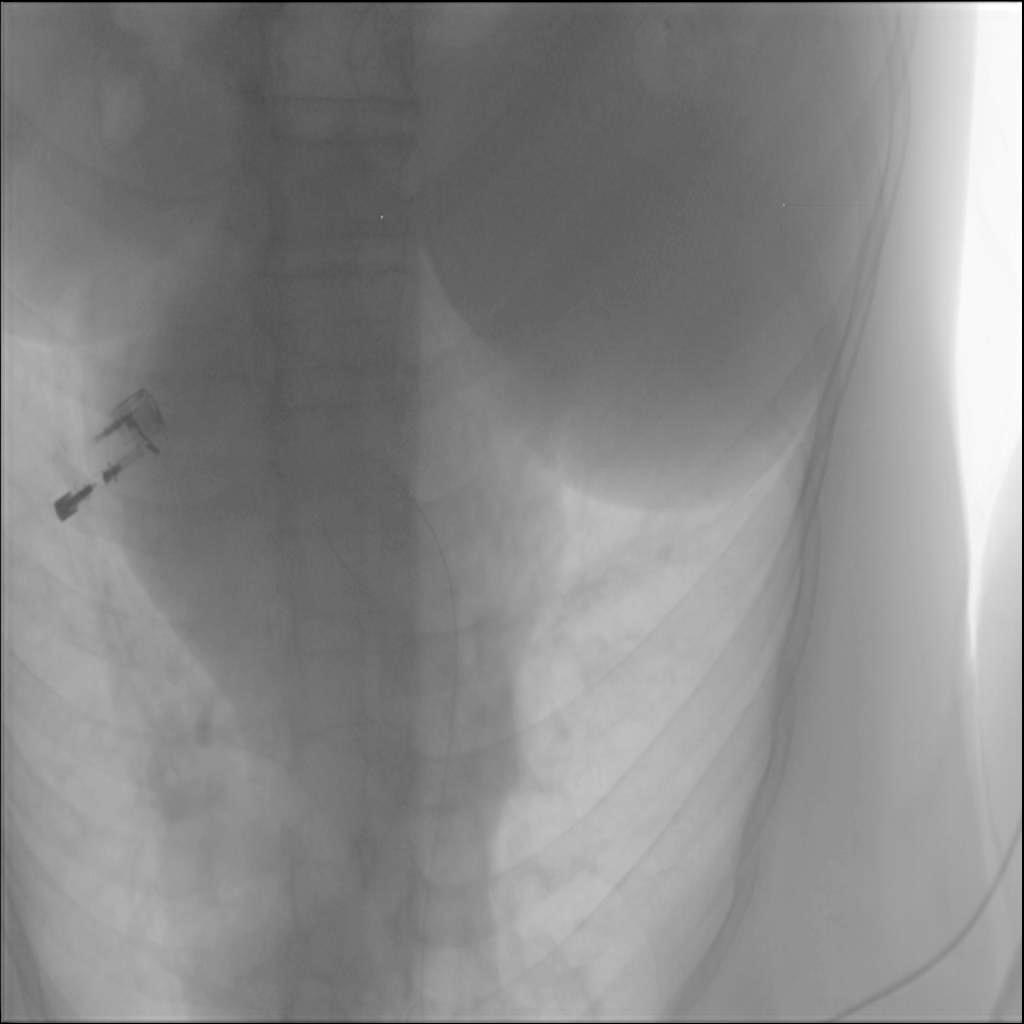}
			\scriptsize{Ours}
		\end{minipage}
		\begin{minipage}[t]{0.19\textwidth}
			\centering
			\includegraphics[width=1\textwidth]{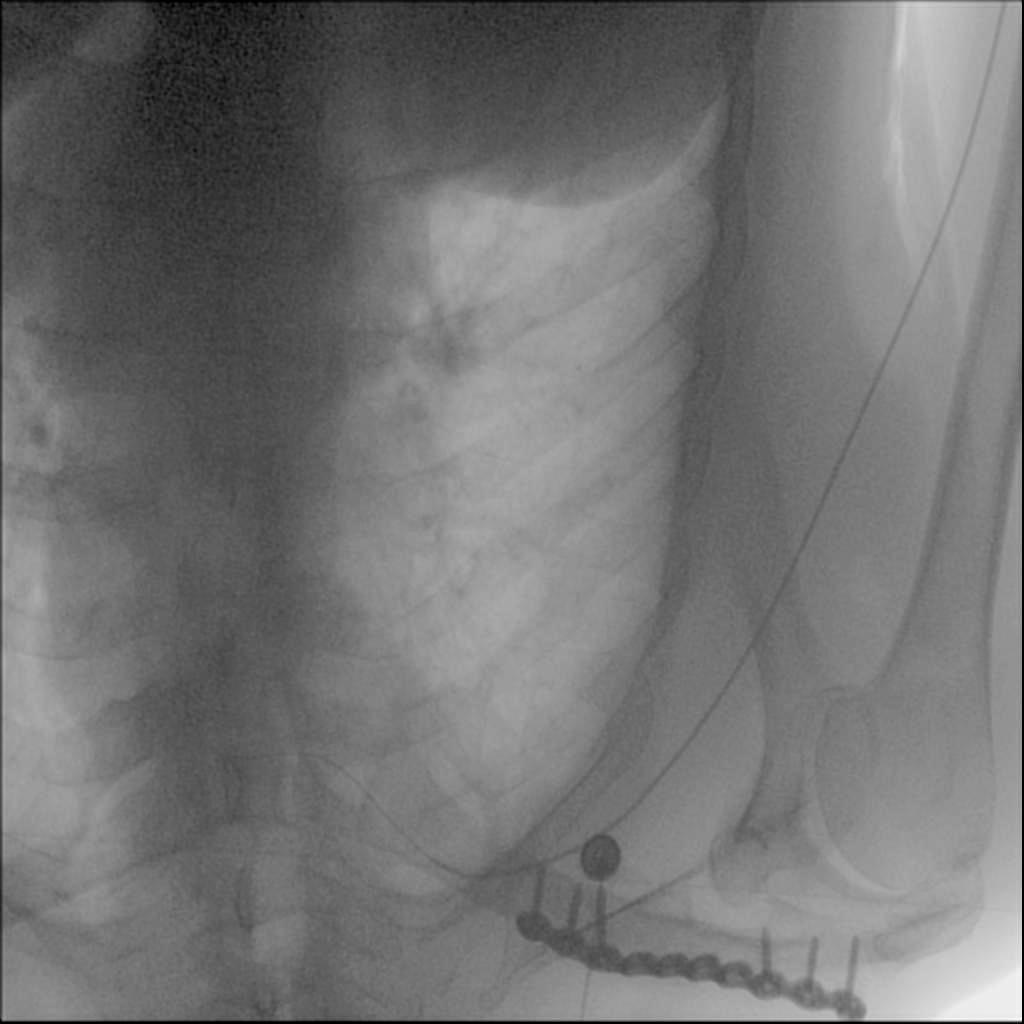}
			\includegraphics[width=1\textwidth]{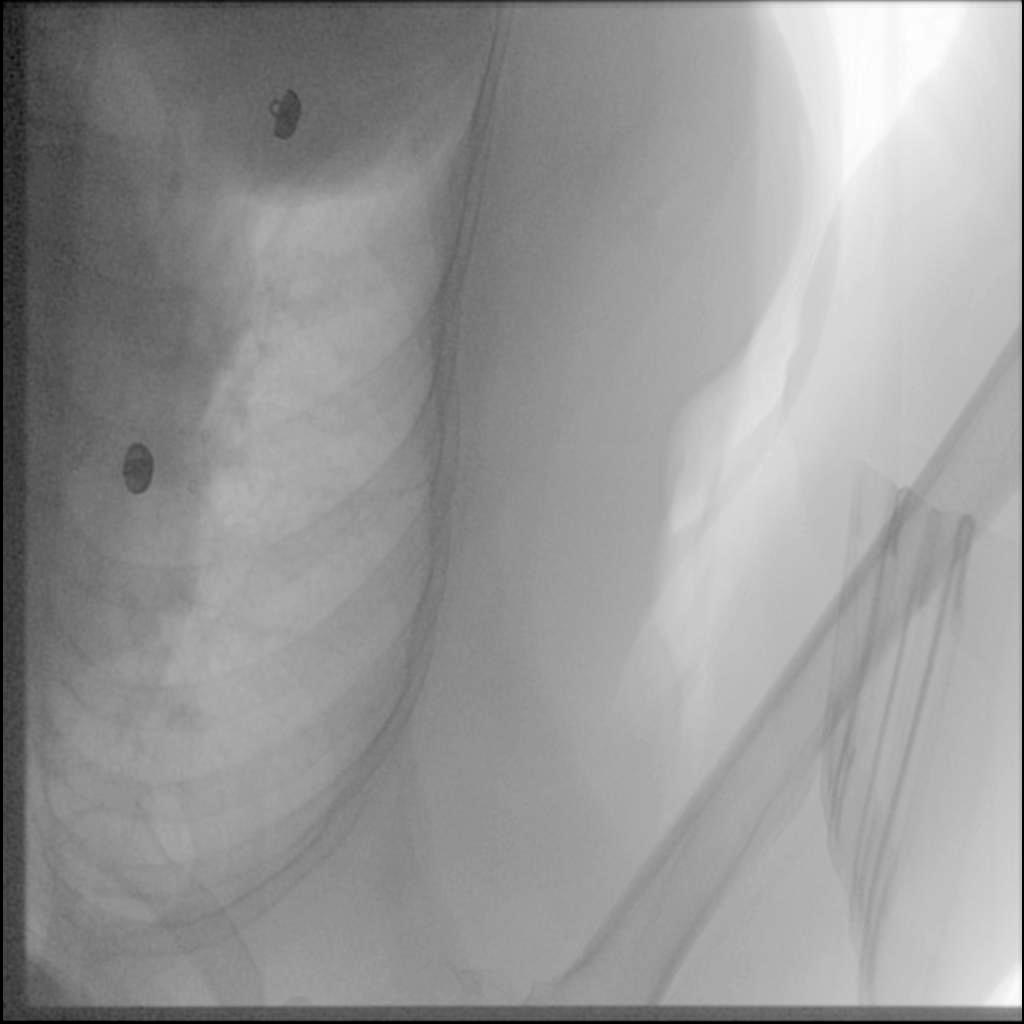}
			\includegraphics[width=1\textwidth]{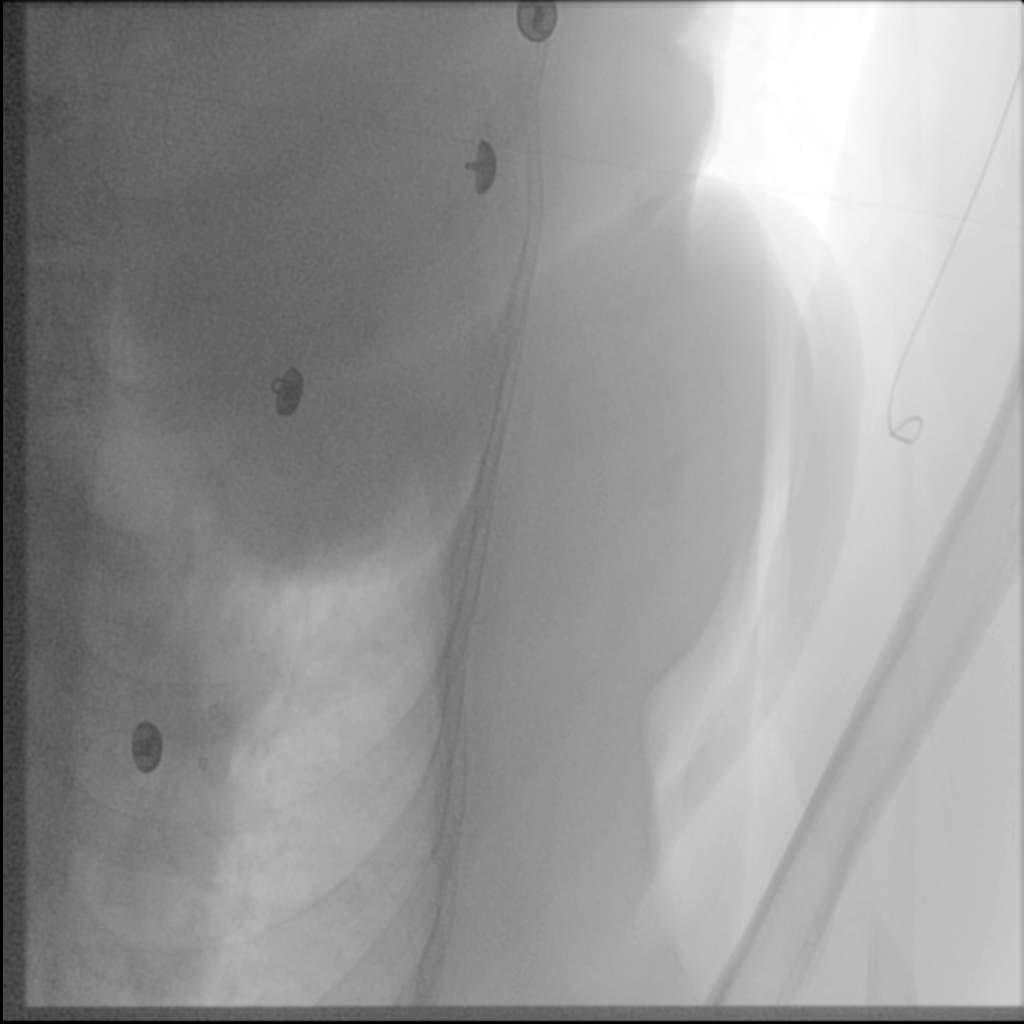}
			\includegraphics[width=1\textwidth]{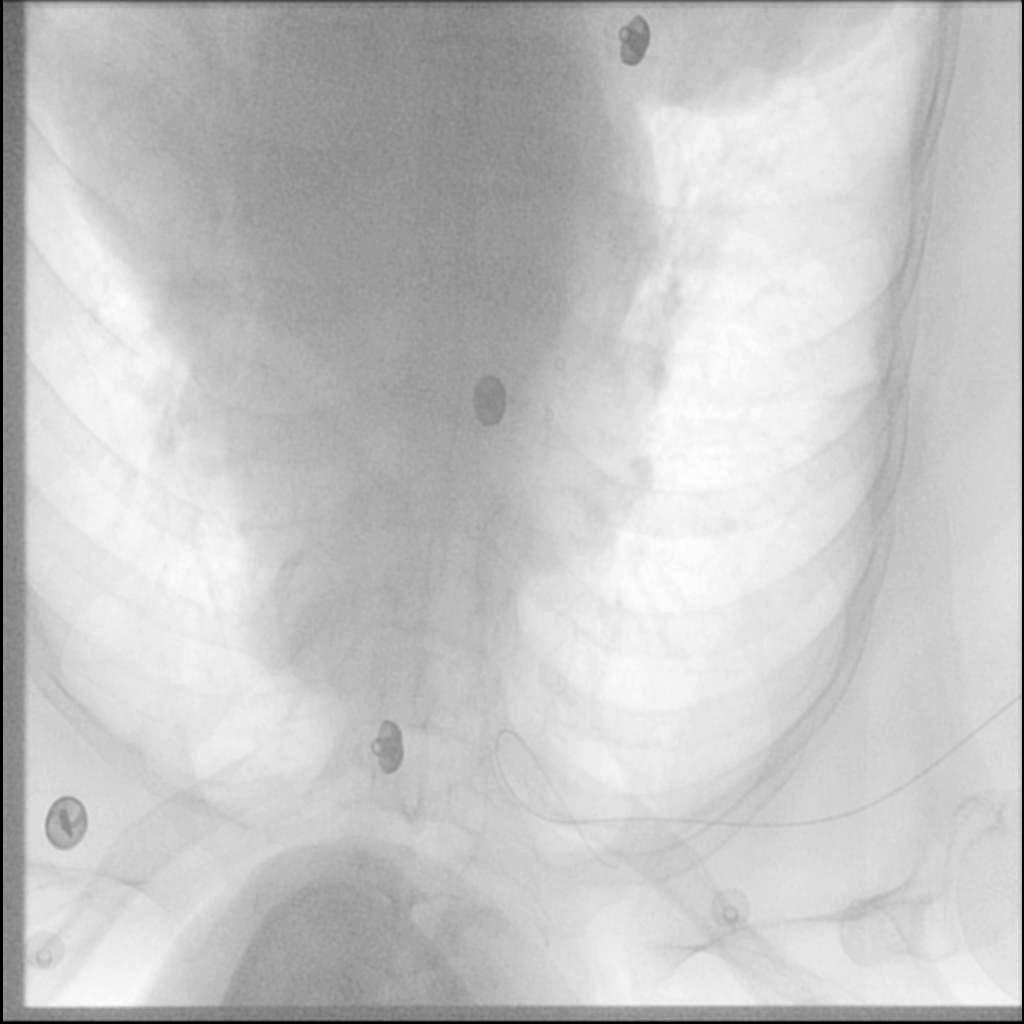}
			\includegraphics[width=1\textwidth]{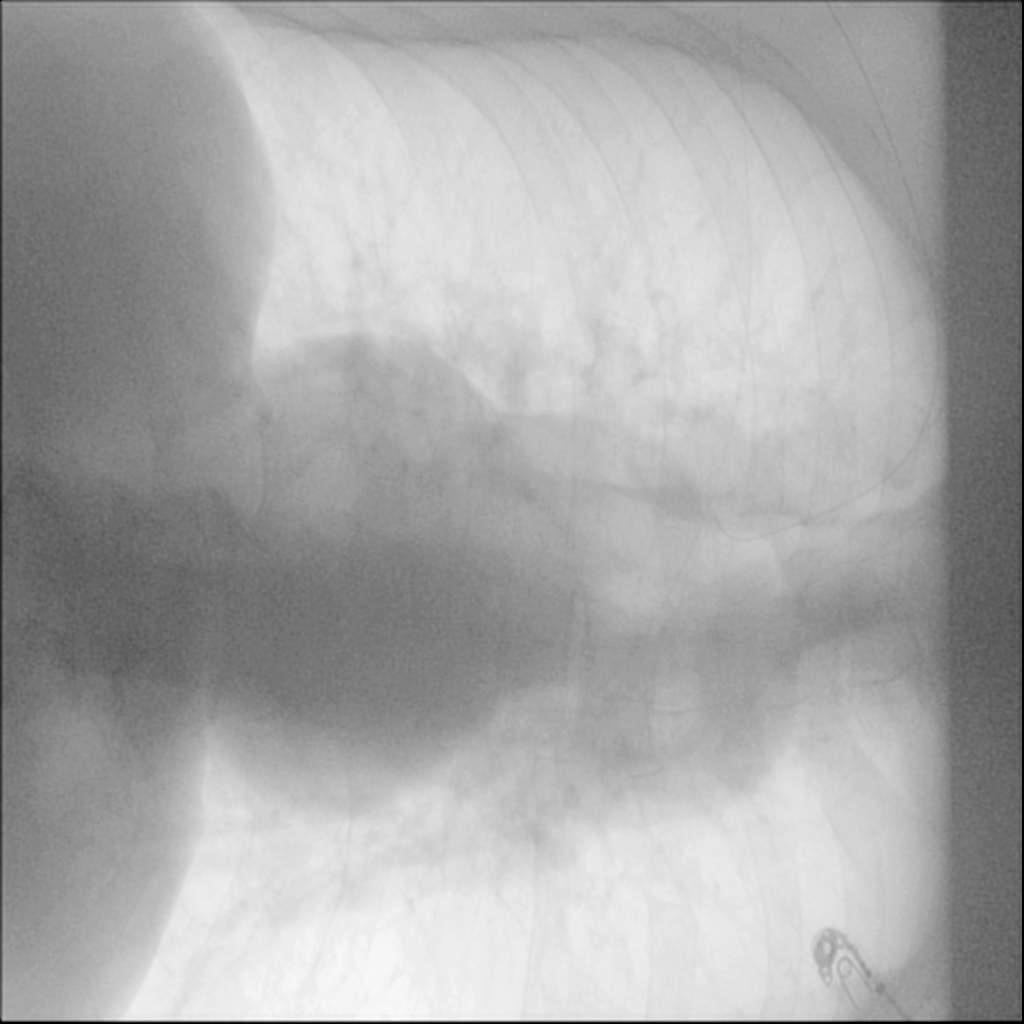}
			\includegraphics[width=1\textwidth]{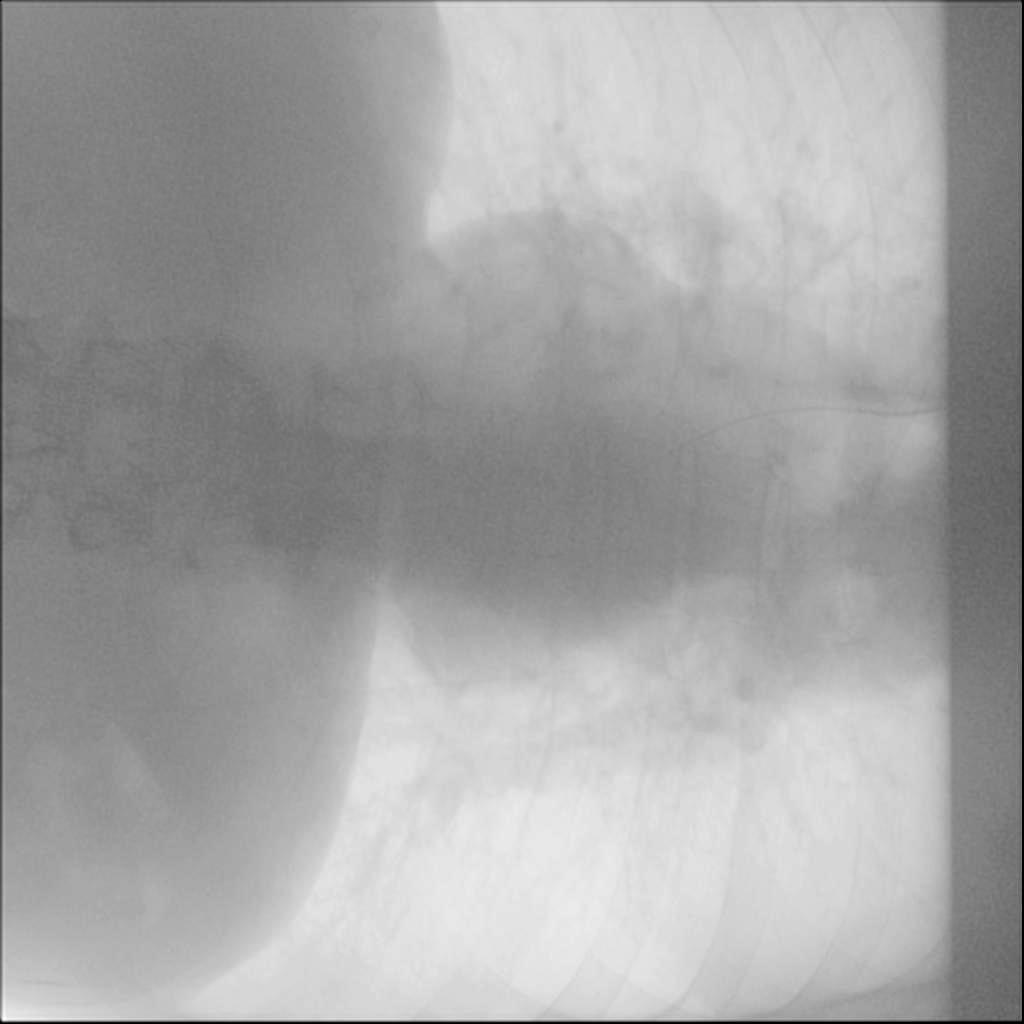}
			\includegraphics[width=1\textwidth]{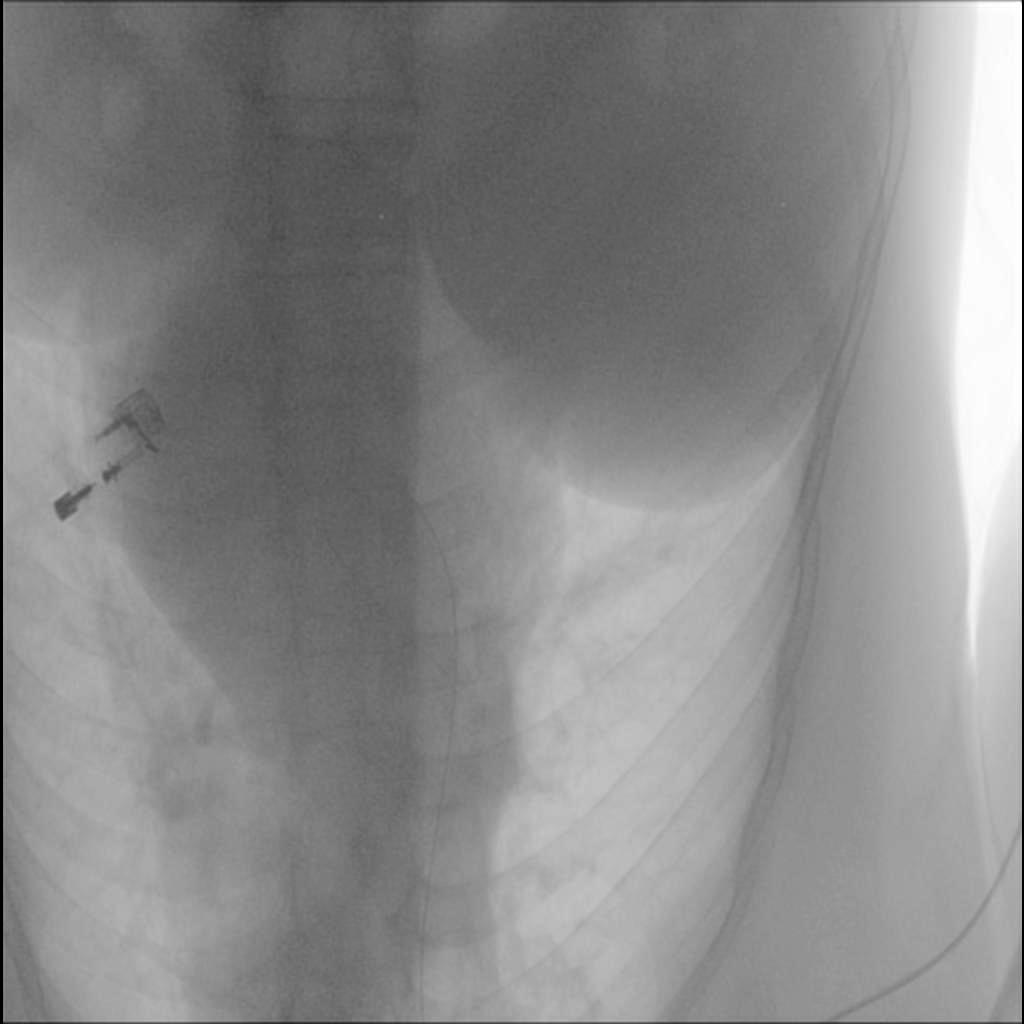}
			\scriptsize{Noise2Self}
		\end{minipage}
		\begin{minipage}[t]{0.19\textwidth}
			\centering
			\includegraphics[width=1\textwidth]{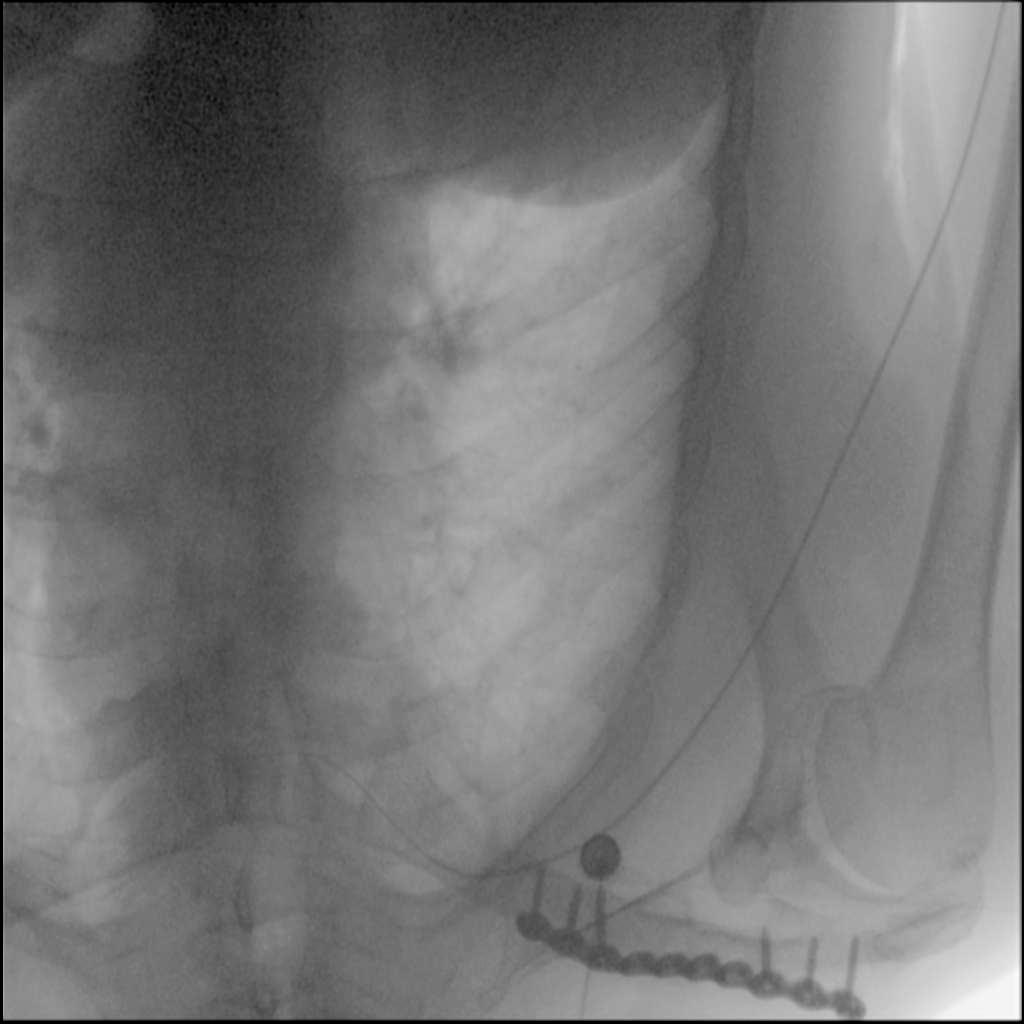}
			\includegraphics[width=1\textwidth]{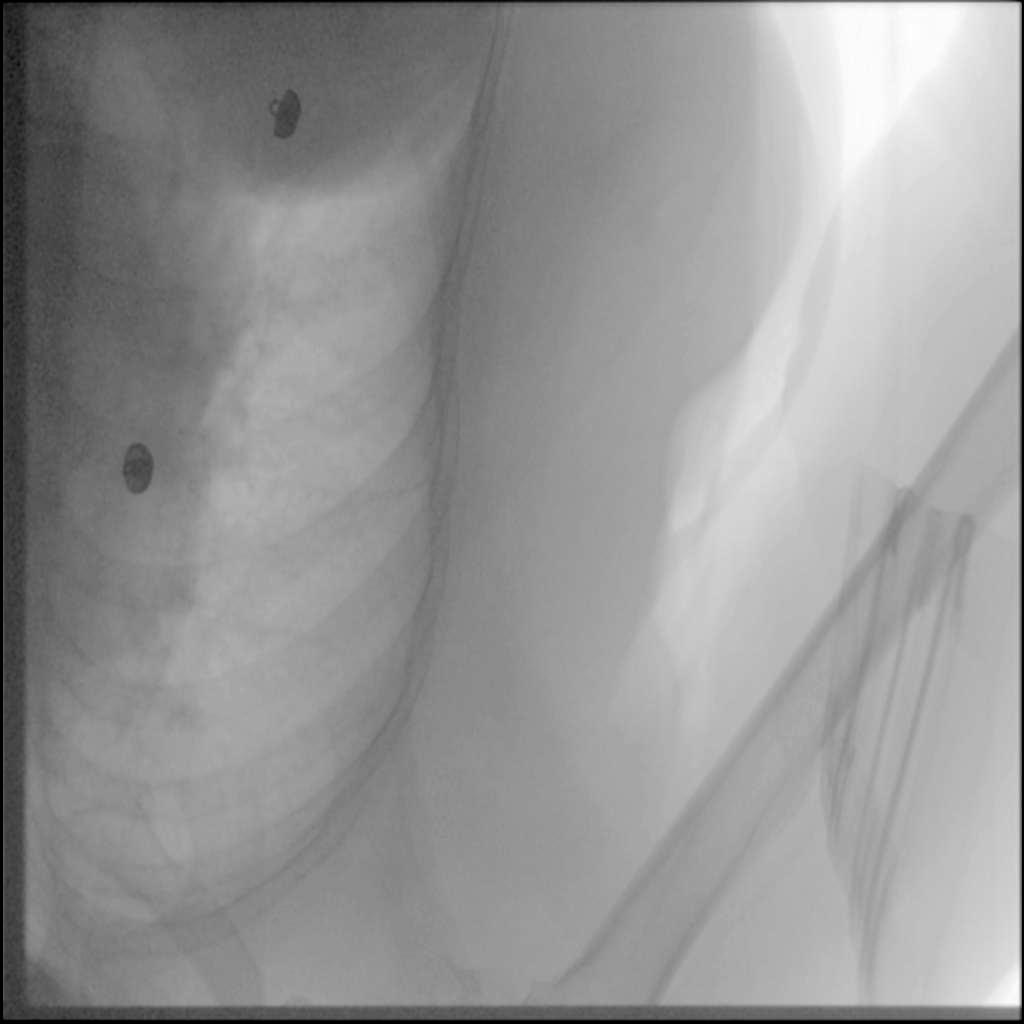}
			\includegraphics[width=1\textwidth]{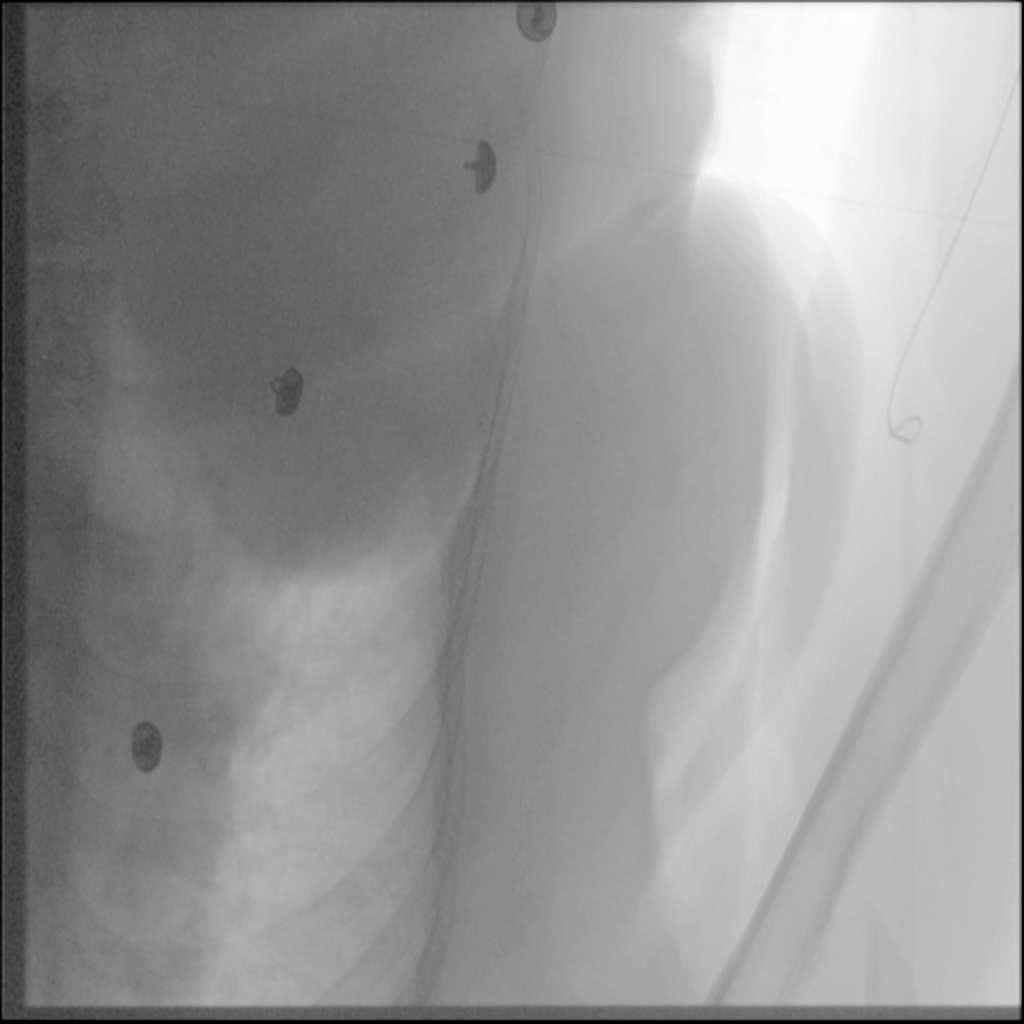}
			\includegraphics[width=1\textwidth]{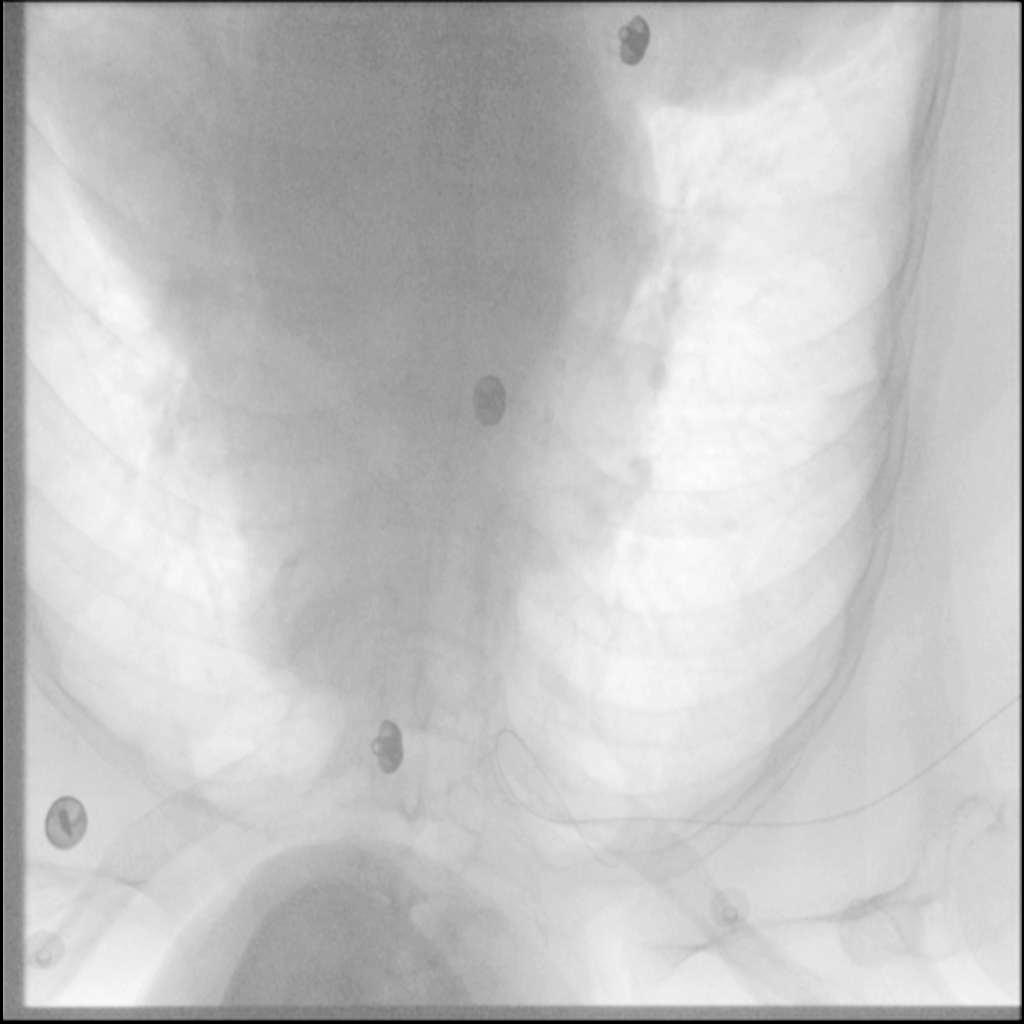}
			\includegraphics[width=1\textwidth]{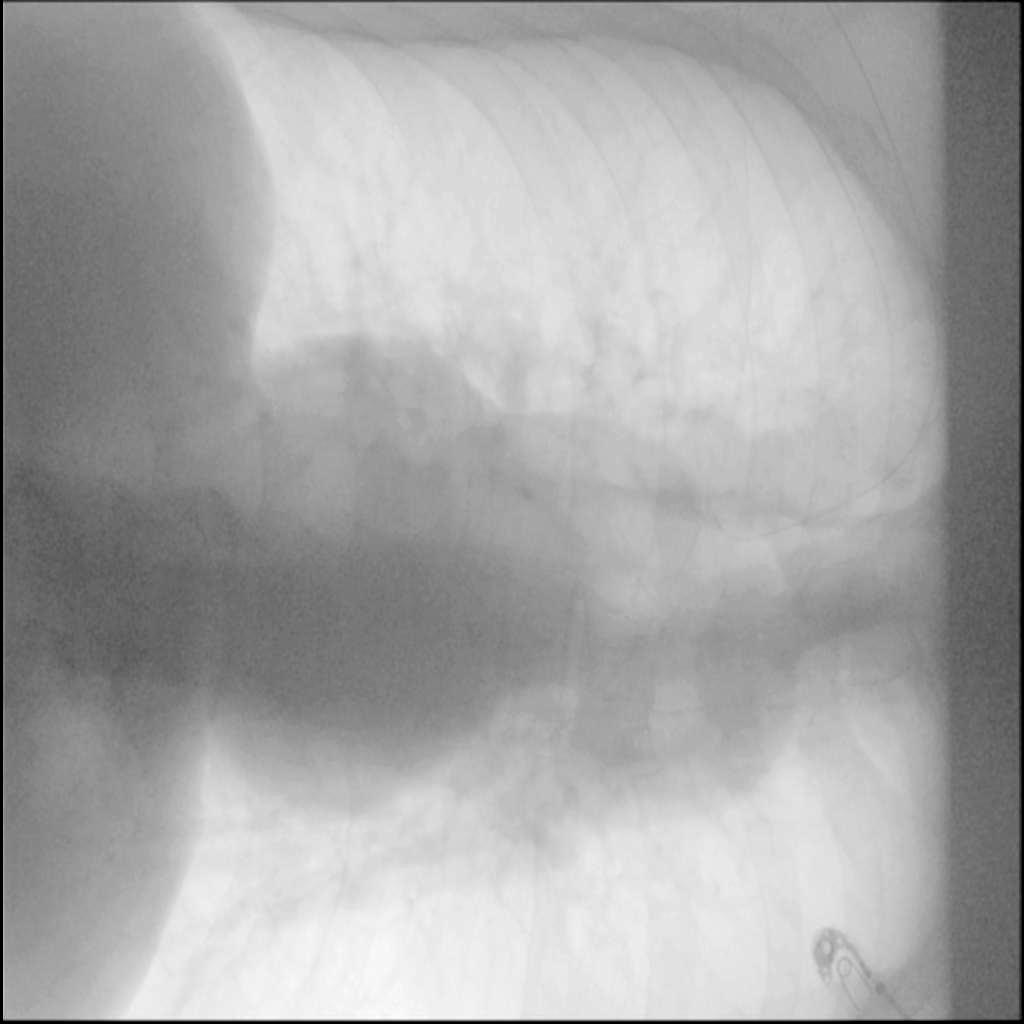}
			\includegraphics[width=1\textwidth]{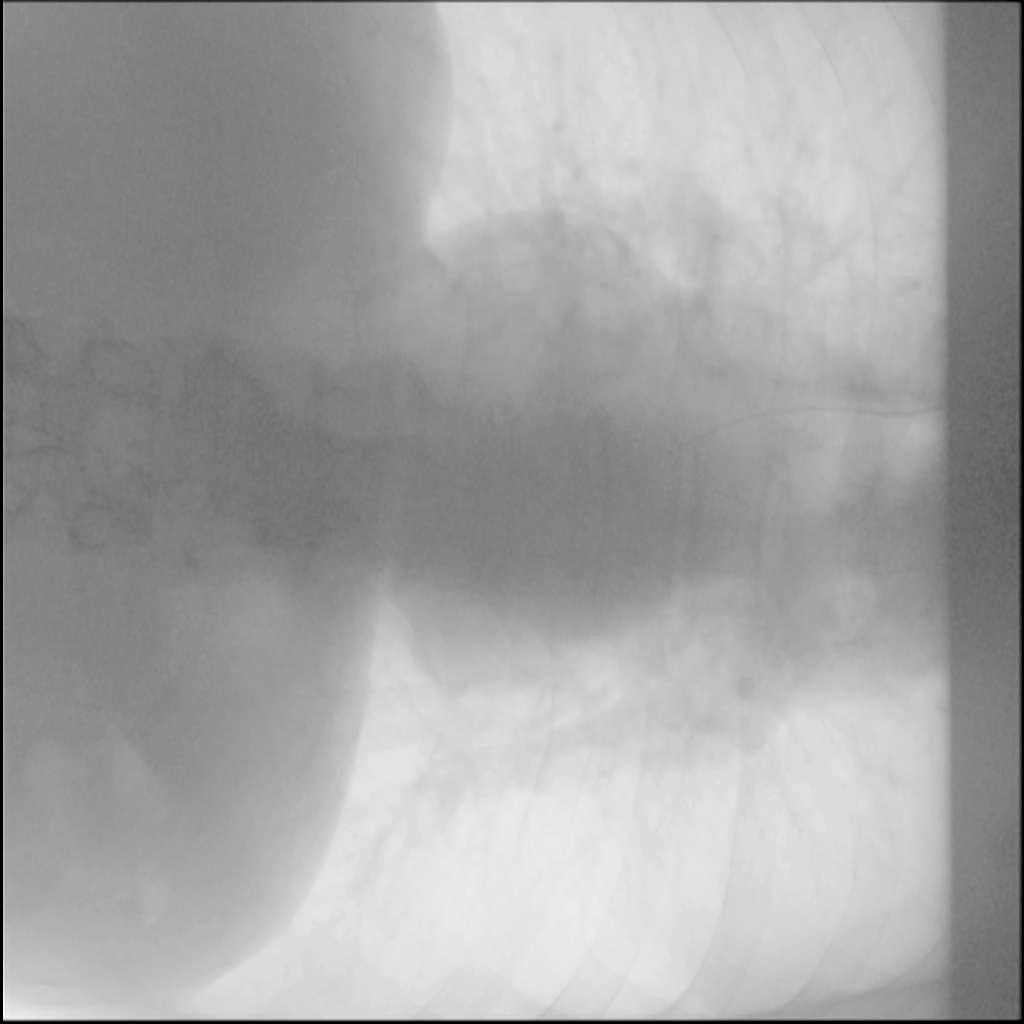}
			\includegraphics[width=1\textwidth]{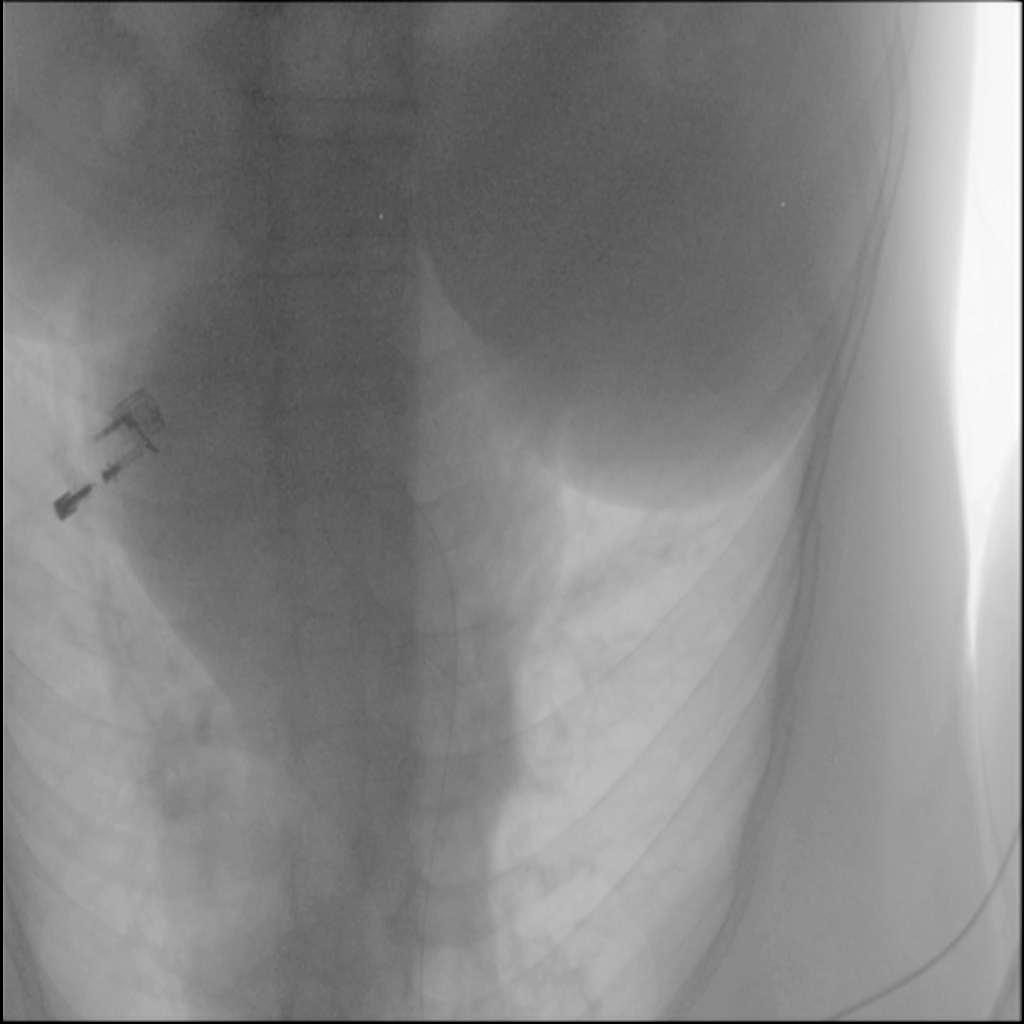}
			\scriptsize{Noise2Void}
		\end{minipage}
		\begin{minipage}[t]{0.19\textwidth}
			\centering
			\includegraphics[width=1\textwidth]{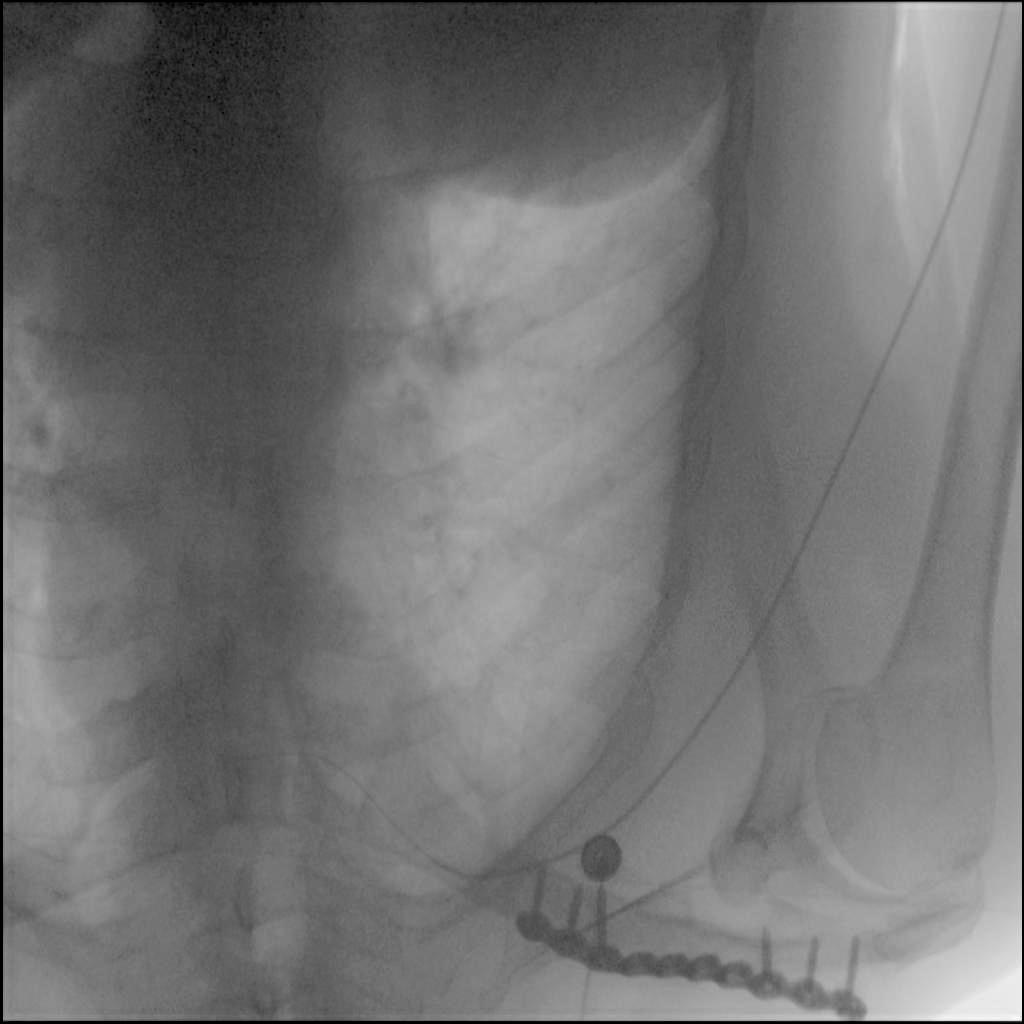}
			\includegraphics[width=1\textwidth]{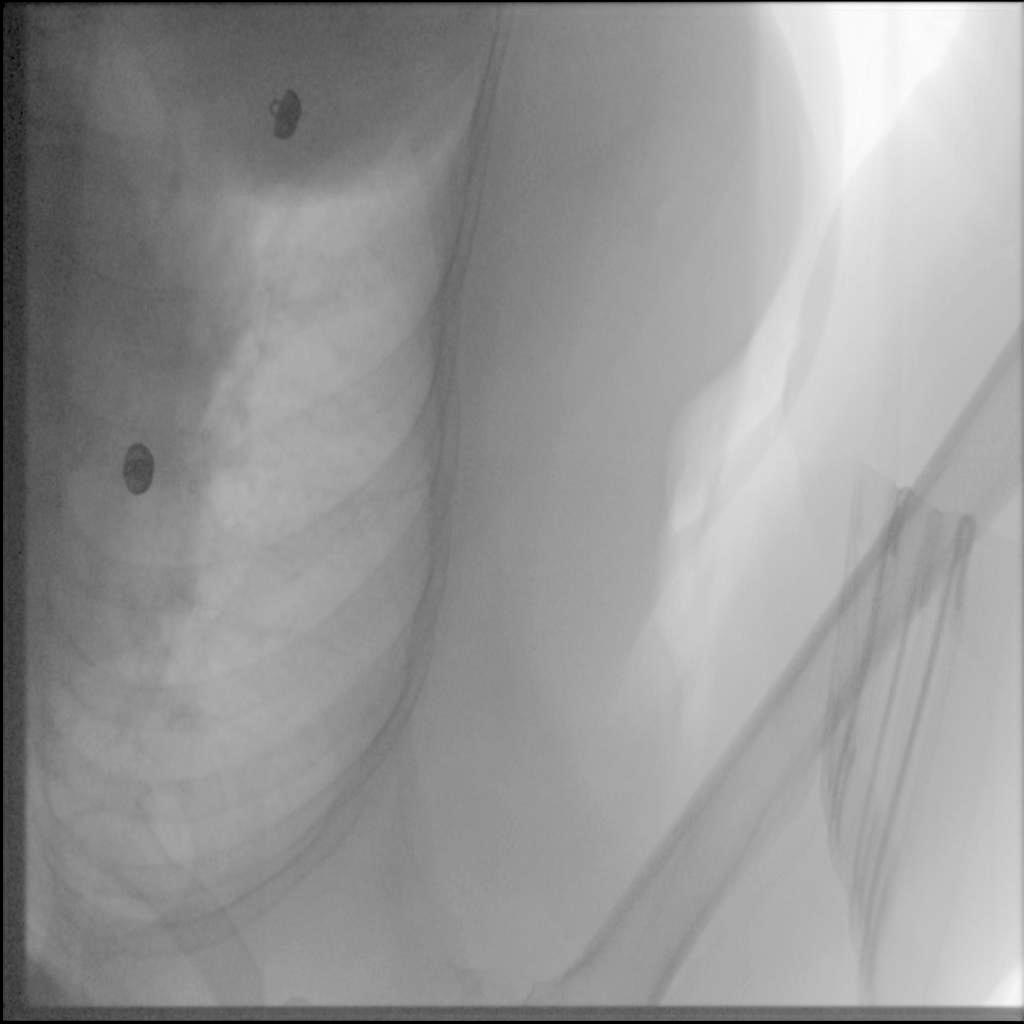}
			\includegraphics[width=1\textwidth]{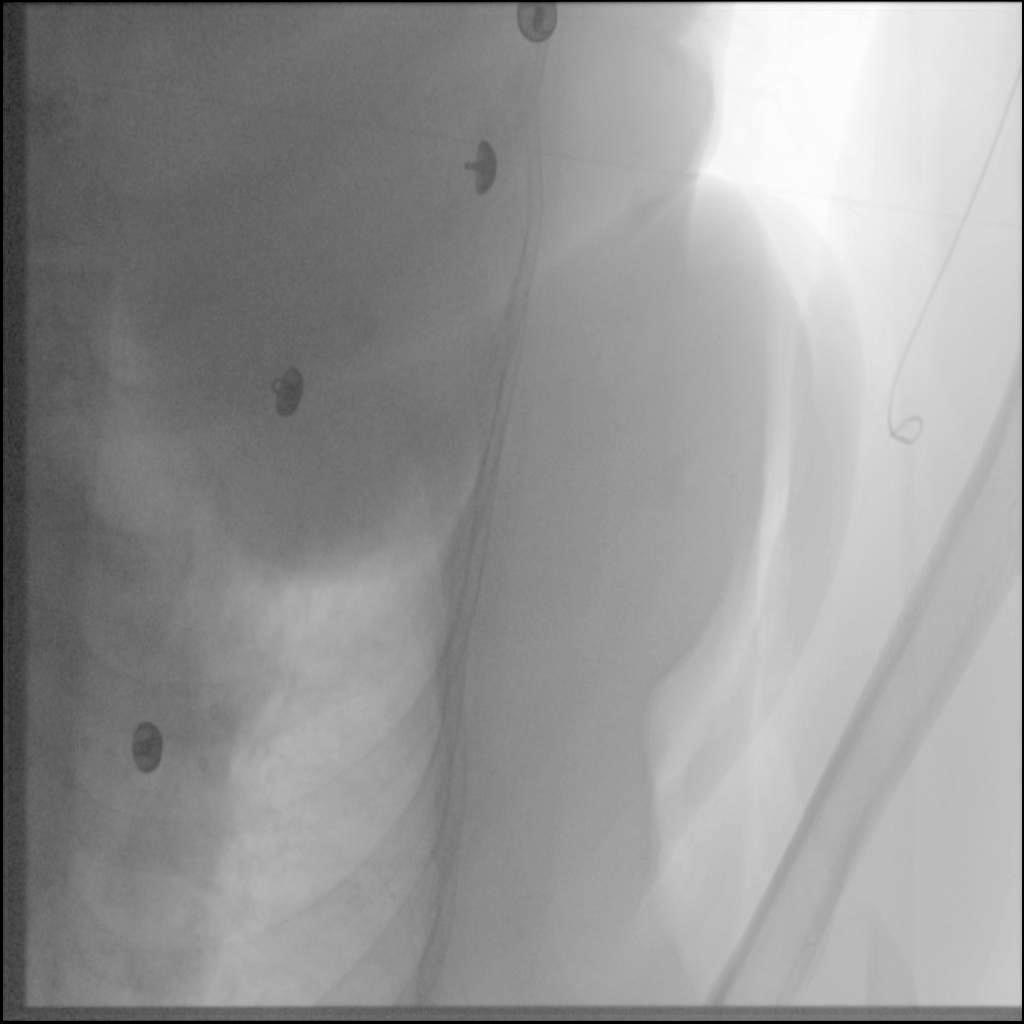}
			\includegraphics[width=1\textwidth]{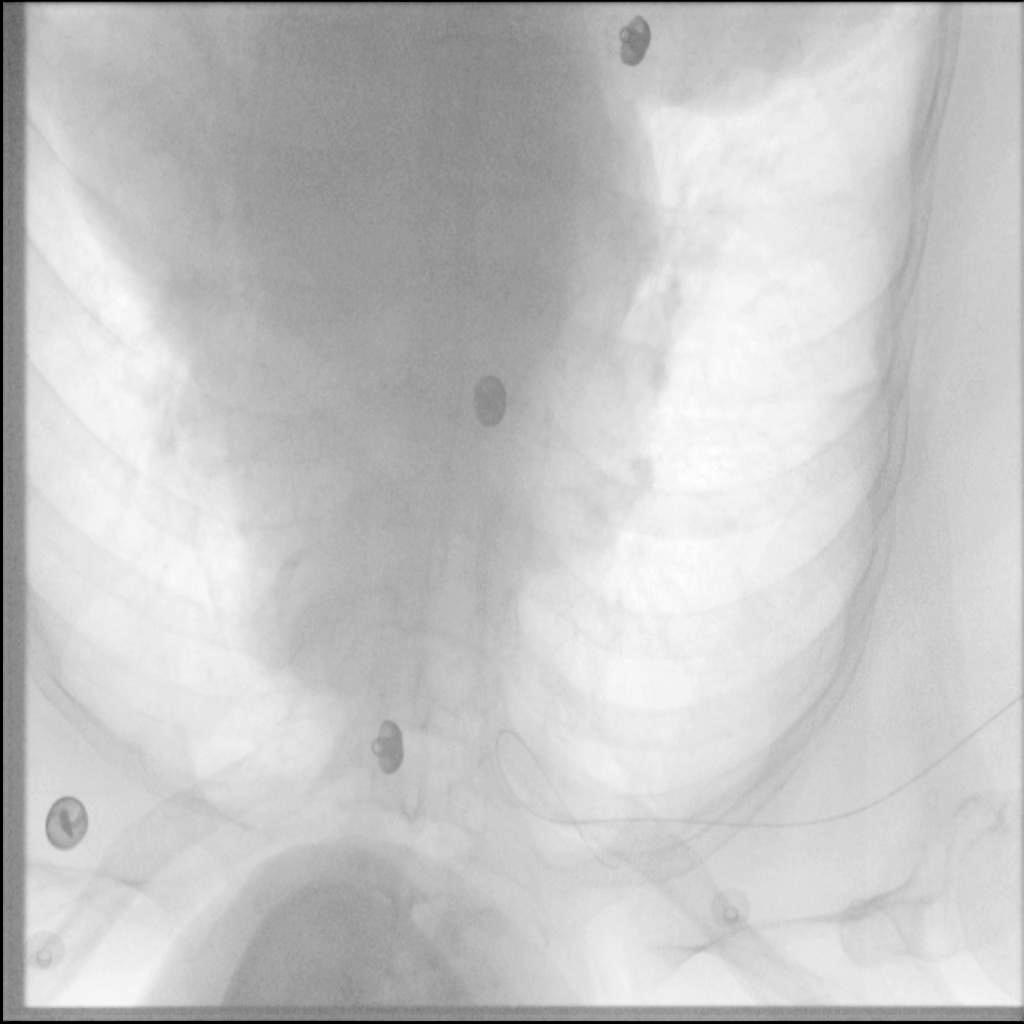}
			\includegraphics[width=1\textwidth]{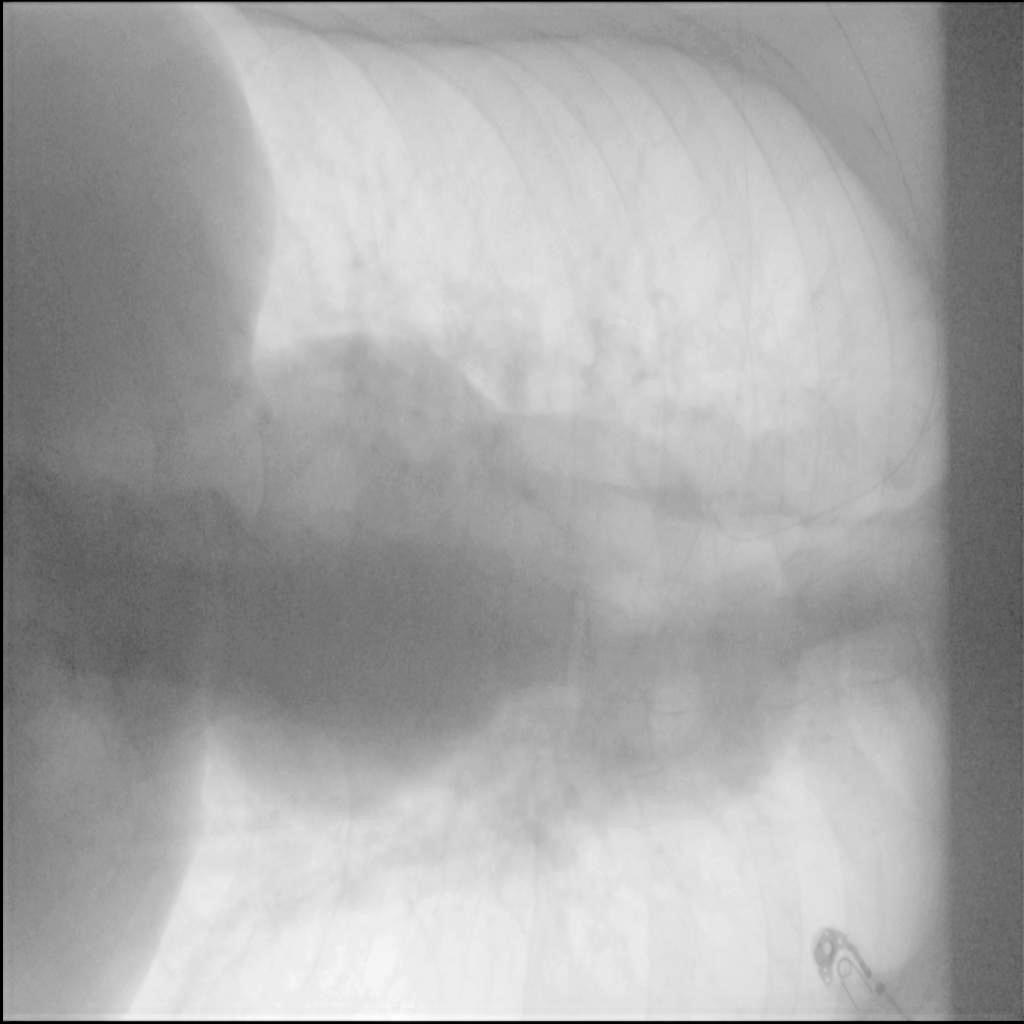}
			\includegraphics[width=1\textwidth]{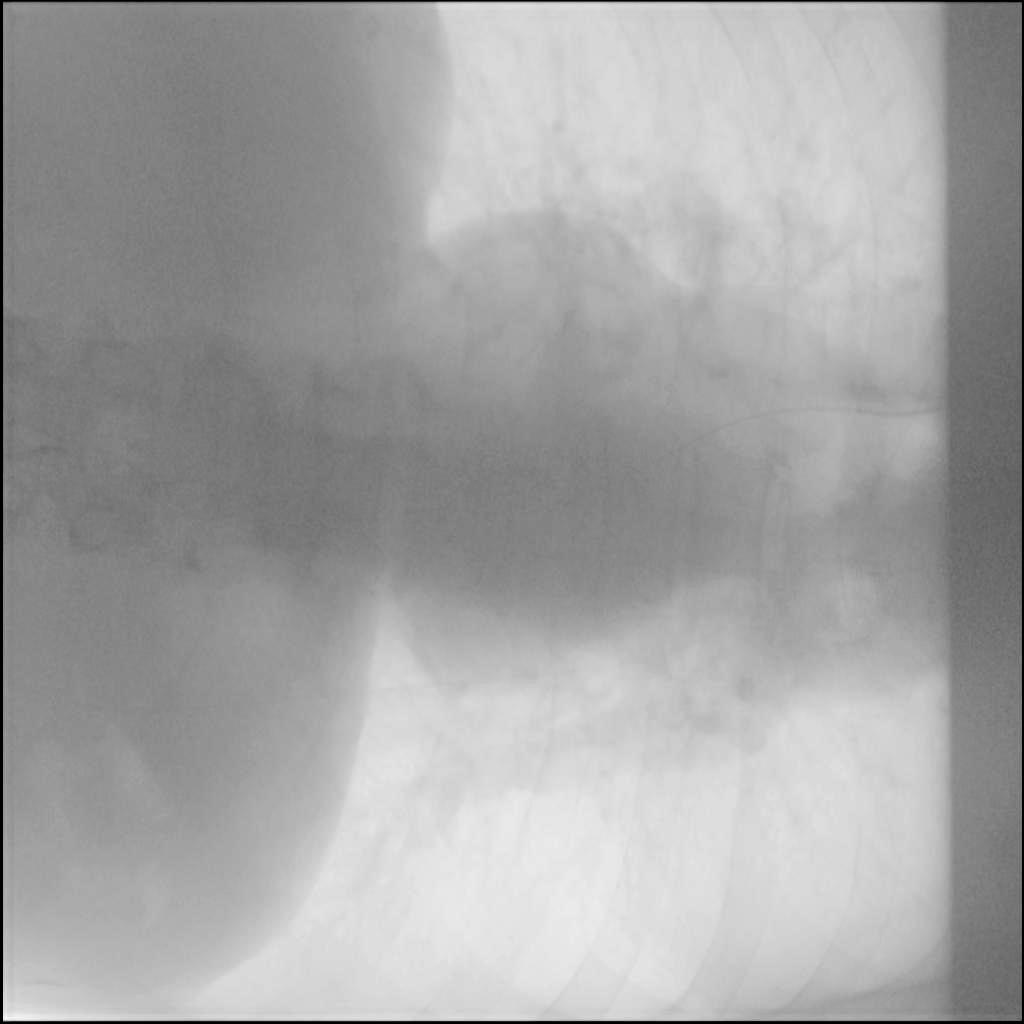}
			\includegraphics[width=1\textwidth]{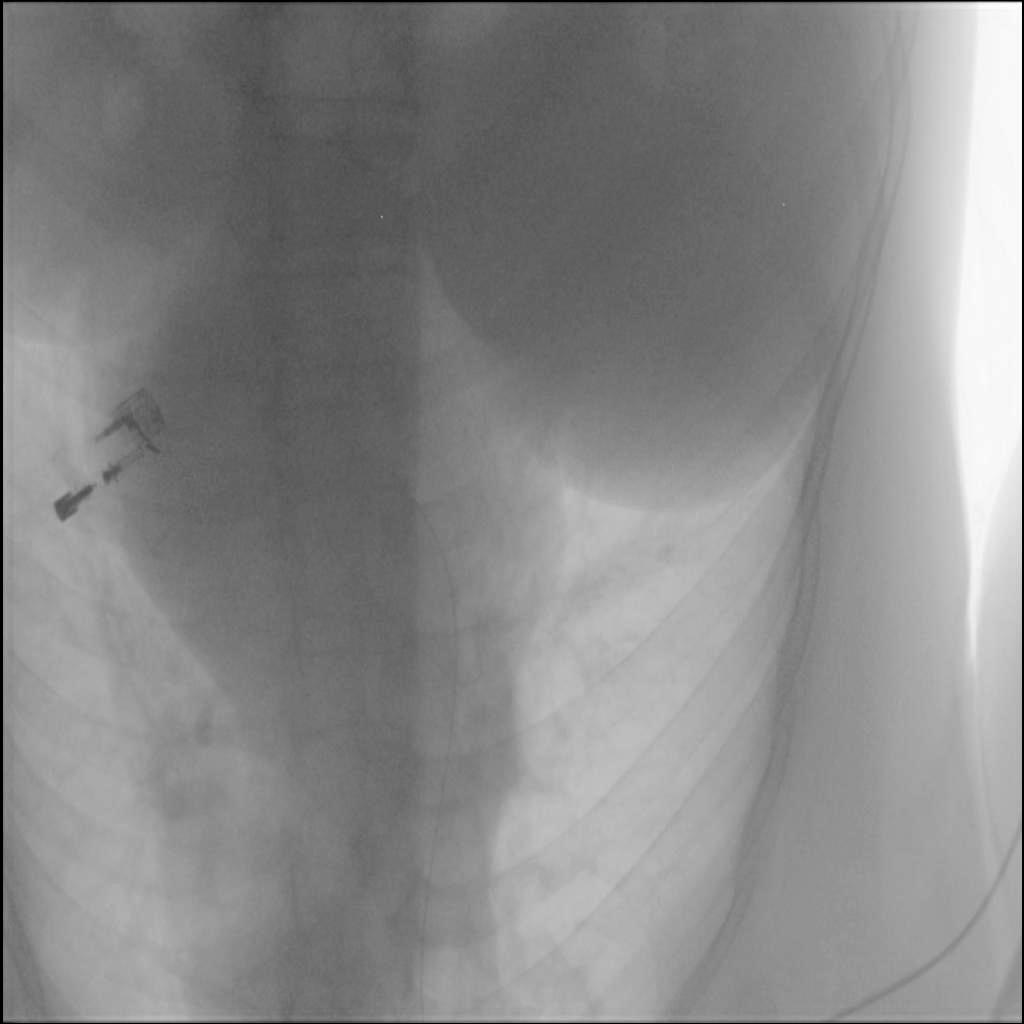}
			\scriptsize{Self2Self}
		\end{minipage}

    \caption{Some groups of clinical samples}
    \label{fig:my_label}
\end{figure}
