# Supplementary material for: Stabilize, Decompose, and Denoise: Self-Supervised Fluoroscopy Denoising
Source: arXiv:2208.14022 source file (2022-08-30)
Supplement: Supplementary file 3 [file t2.tex]

\begin{figure}[!htb]
\small
\centering 

\resizebox{\textwidth}{!}{
    \begin{tabular}{@{}ccccccccl@{}}
    \tiny Input & \tiny GT & \tiny N2V & \tiny N2S & \tiny S2S & \tiny Ours\\
    \includegraphics[width=0.083\textwidth]{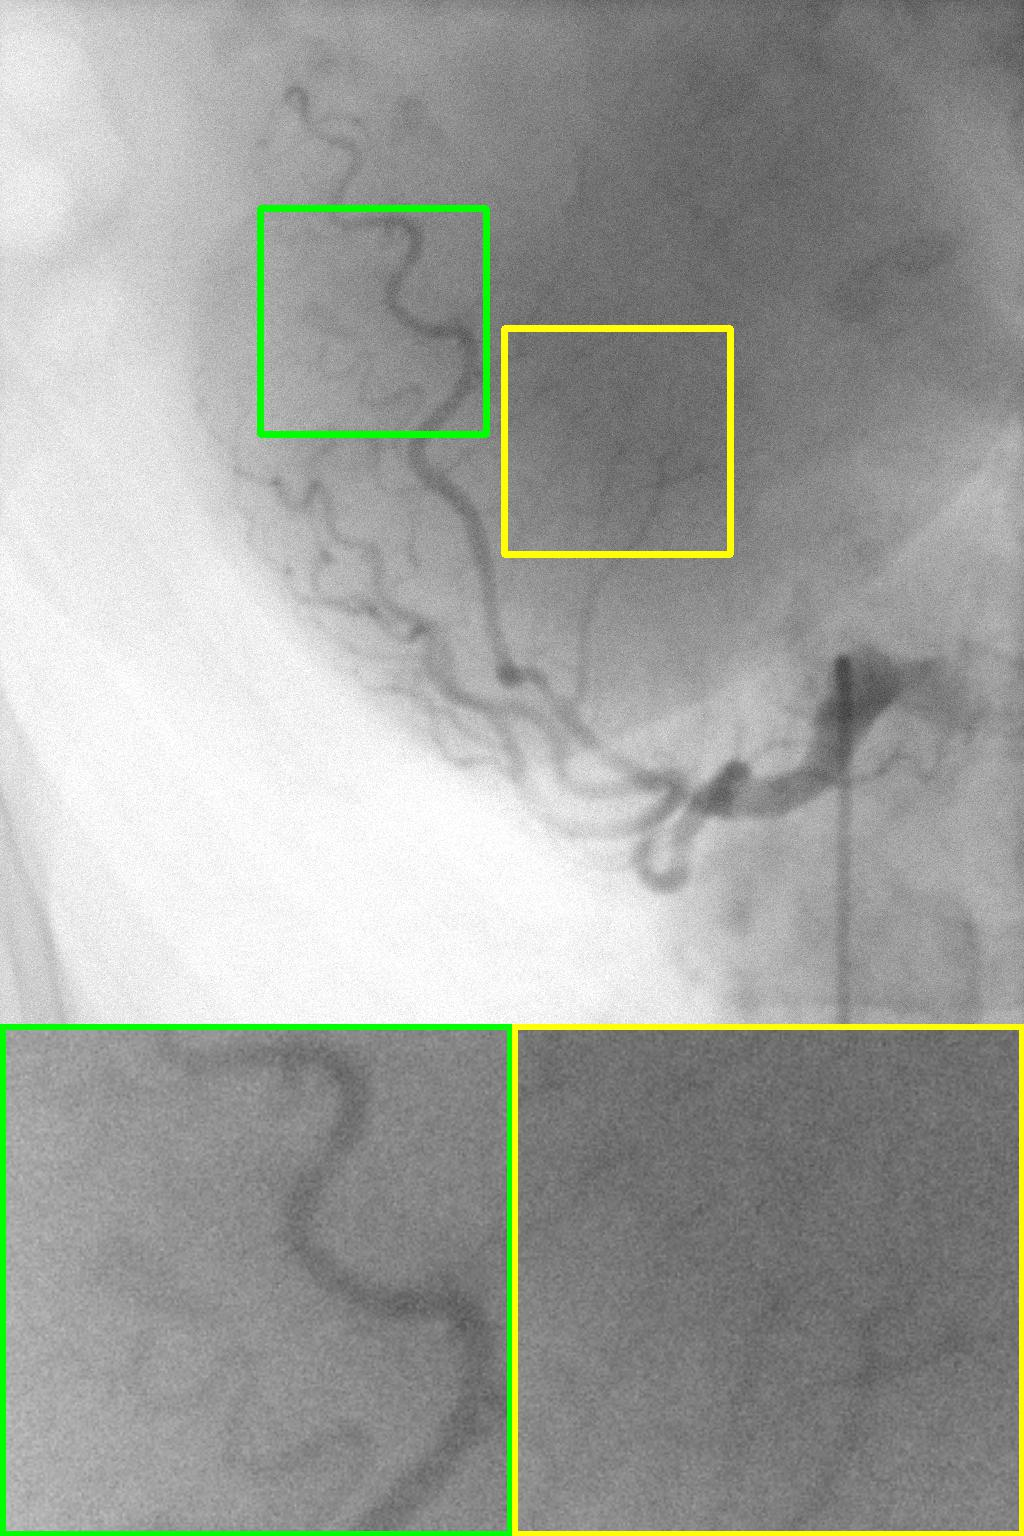} &
    \includegraphics[width=0.083\textwidth]{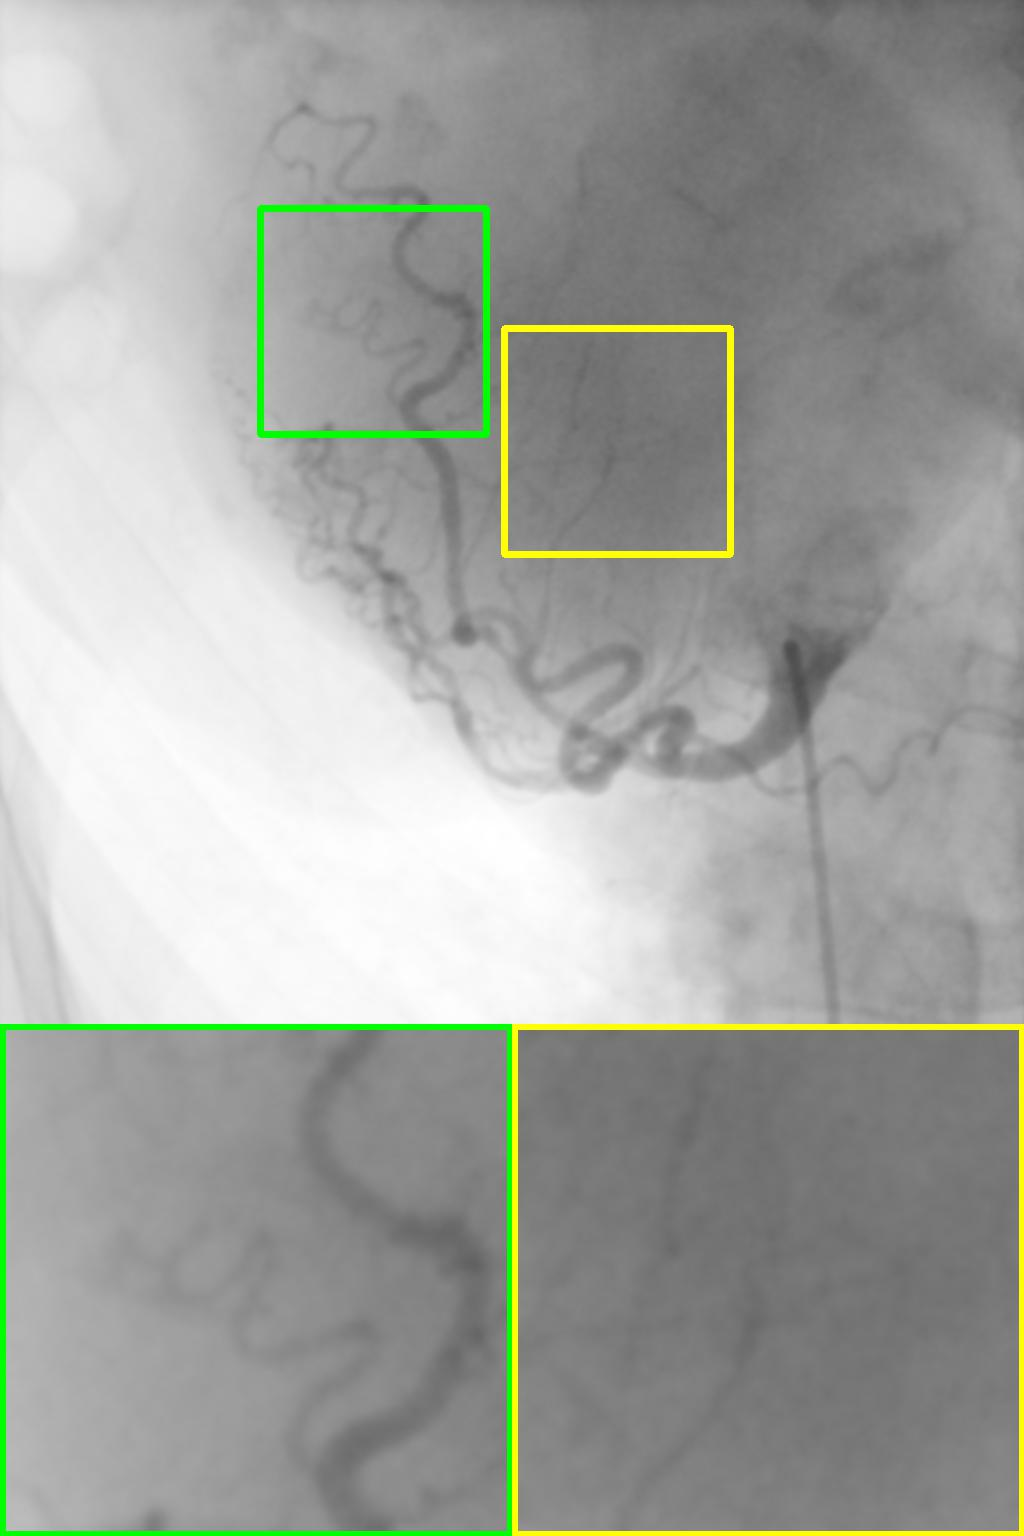} &
    \includegraphics[width=0.083\textwidth]{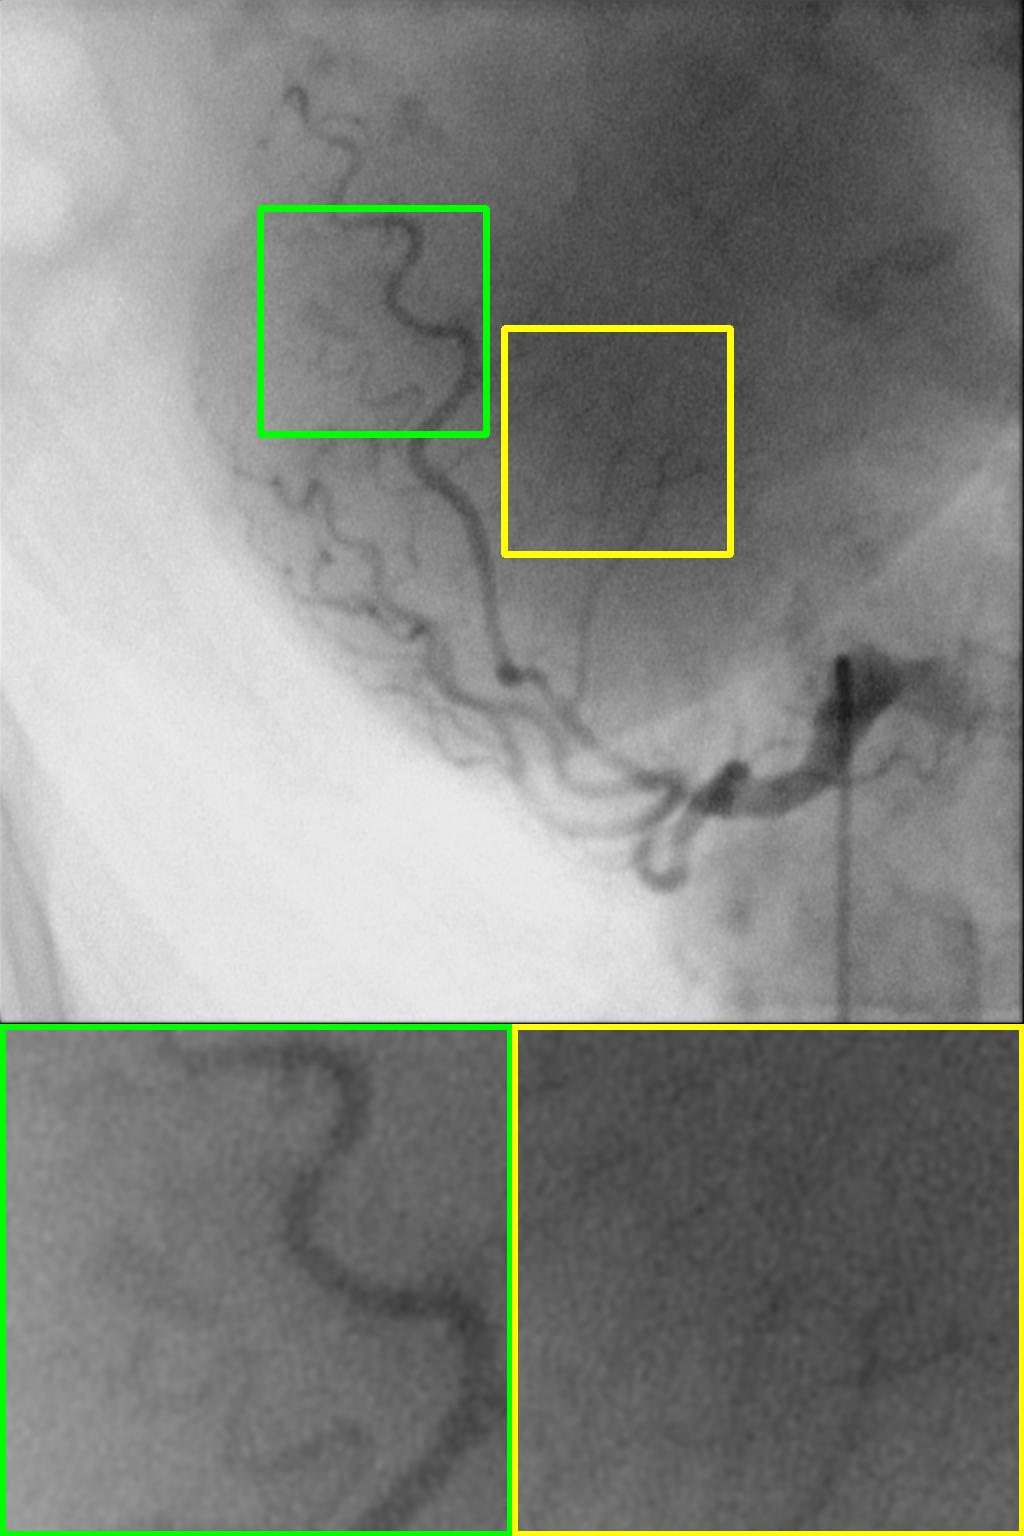} &
    \includegraphics[width=0.083\textwidth]{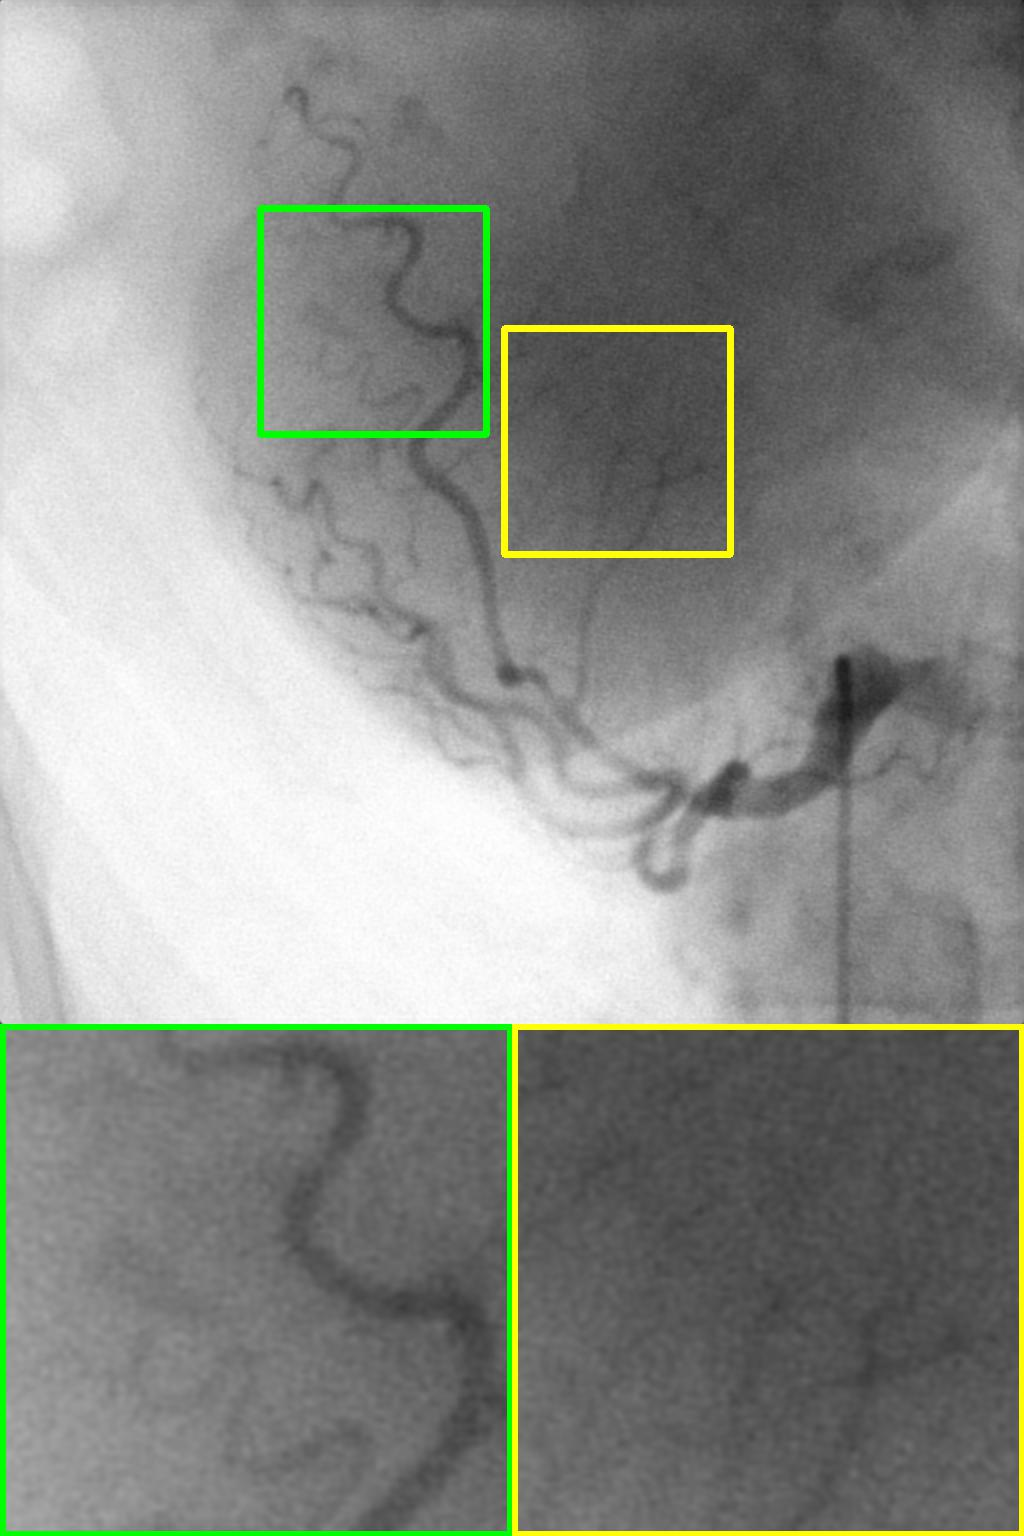}&
    \includegraphics[width=0.083\textwidth]{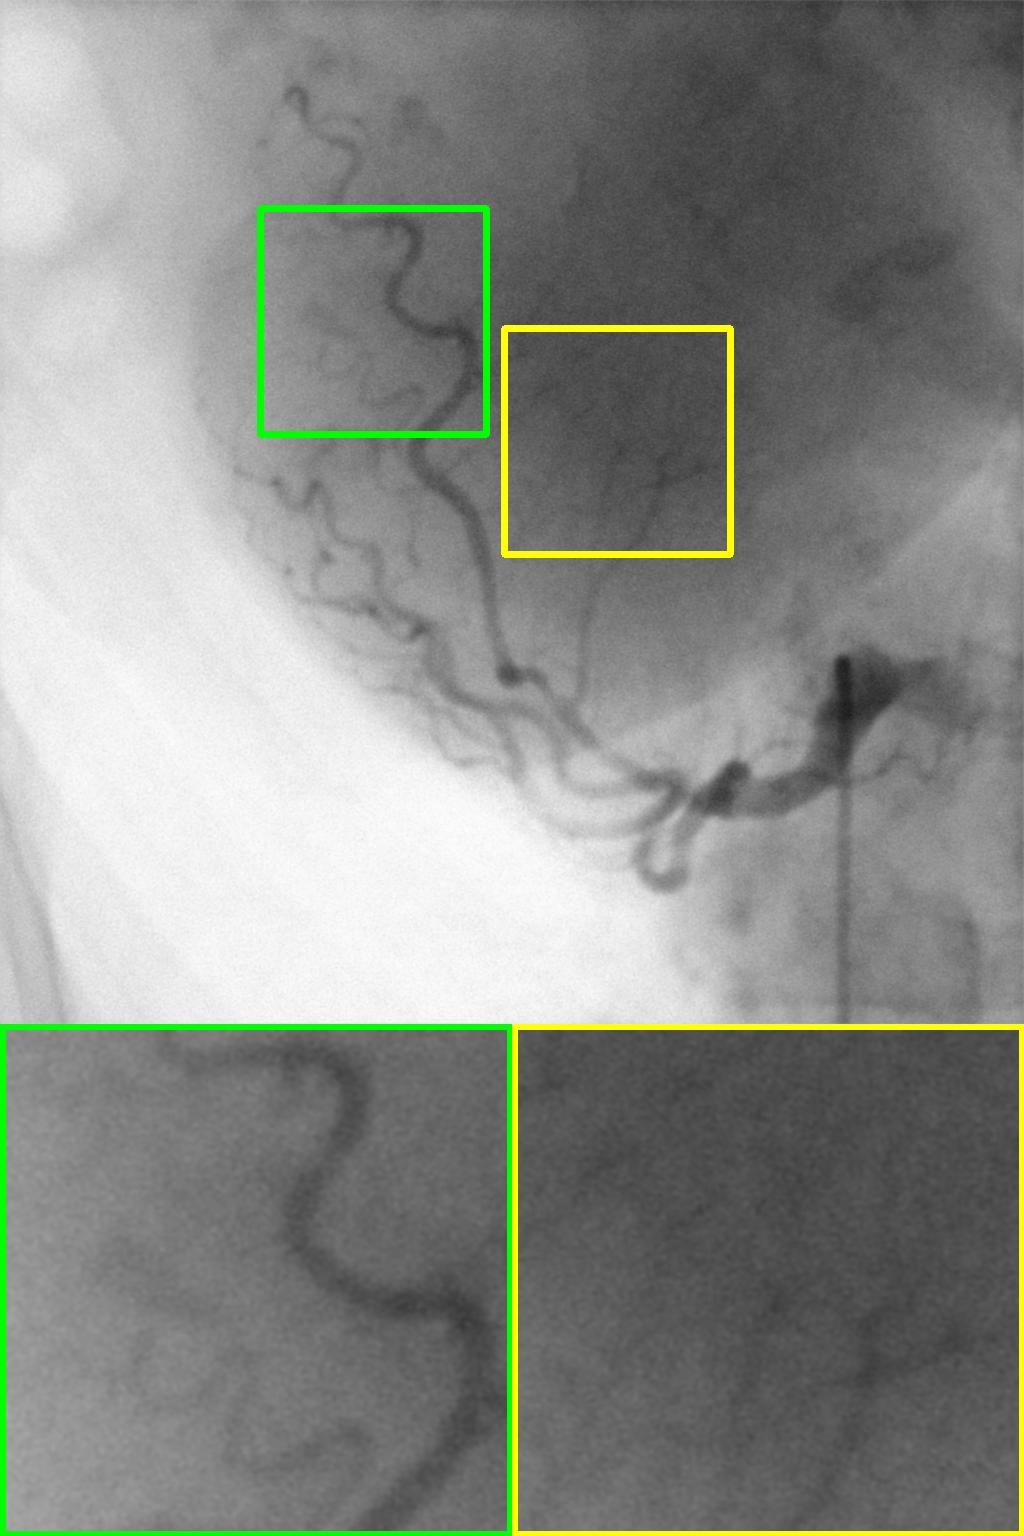}&
    \includegraphics[width=0.083\textwidth]{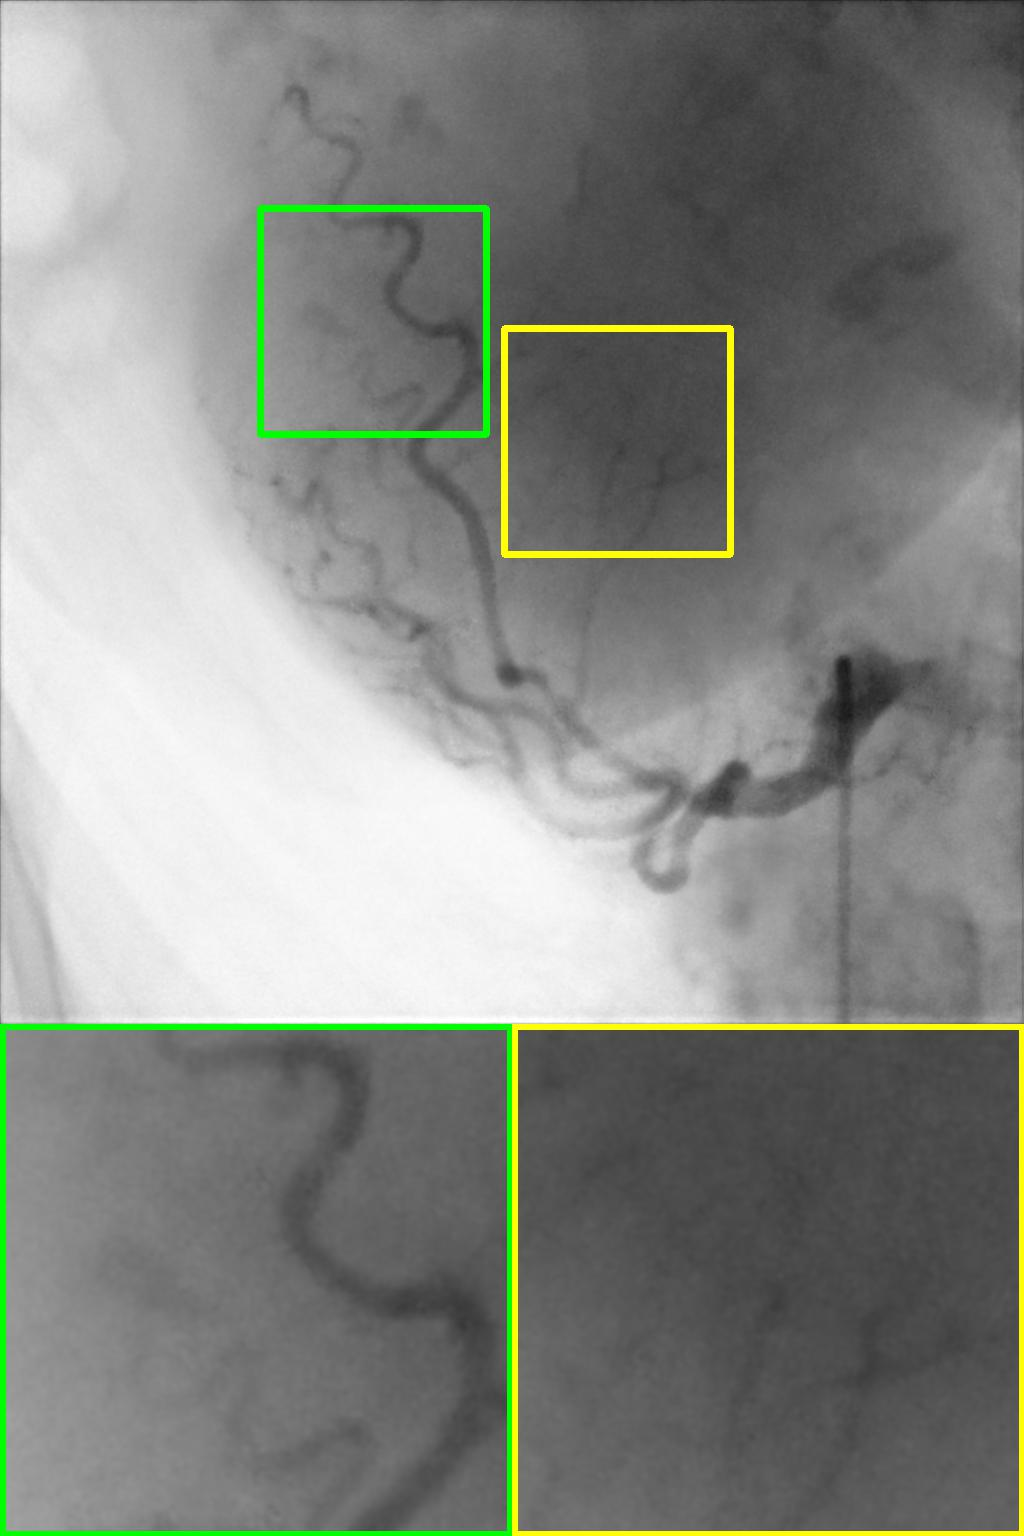}& 
    \\
    
    \includegraphics[width=0.083\textwidth]{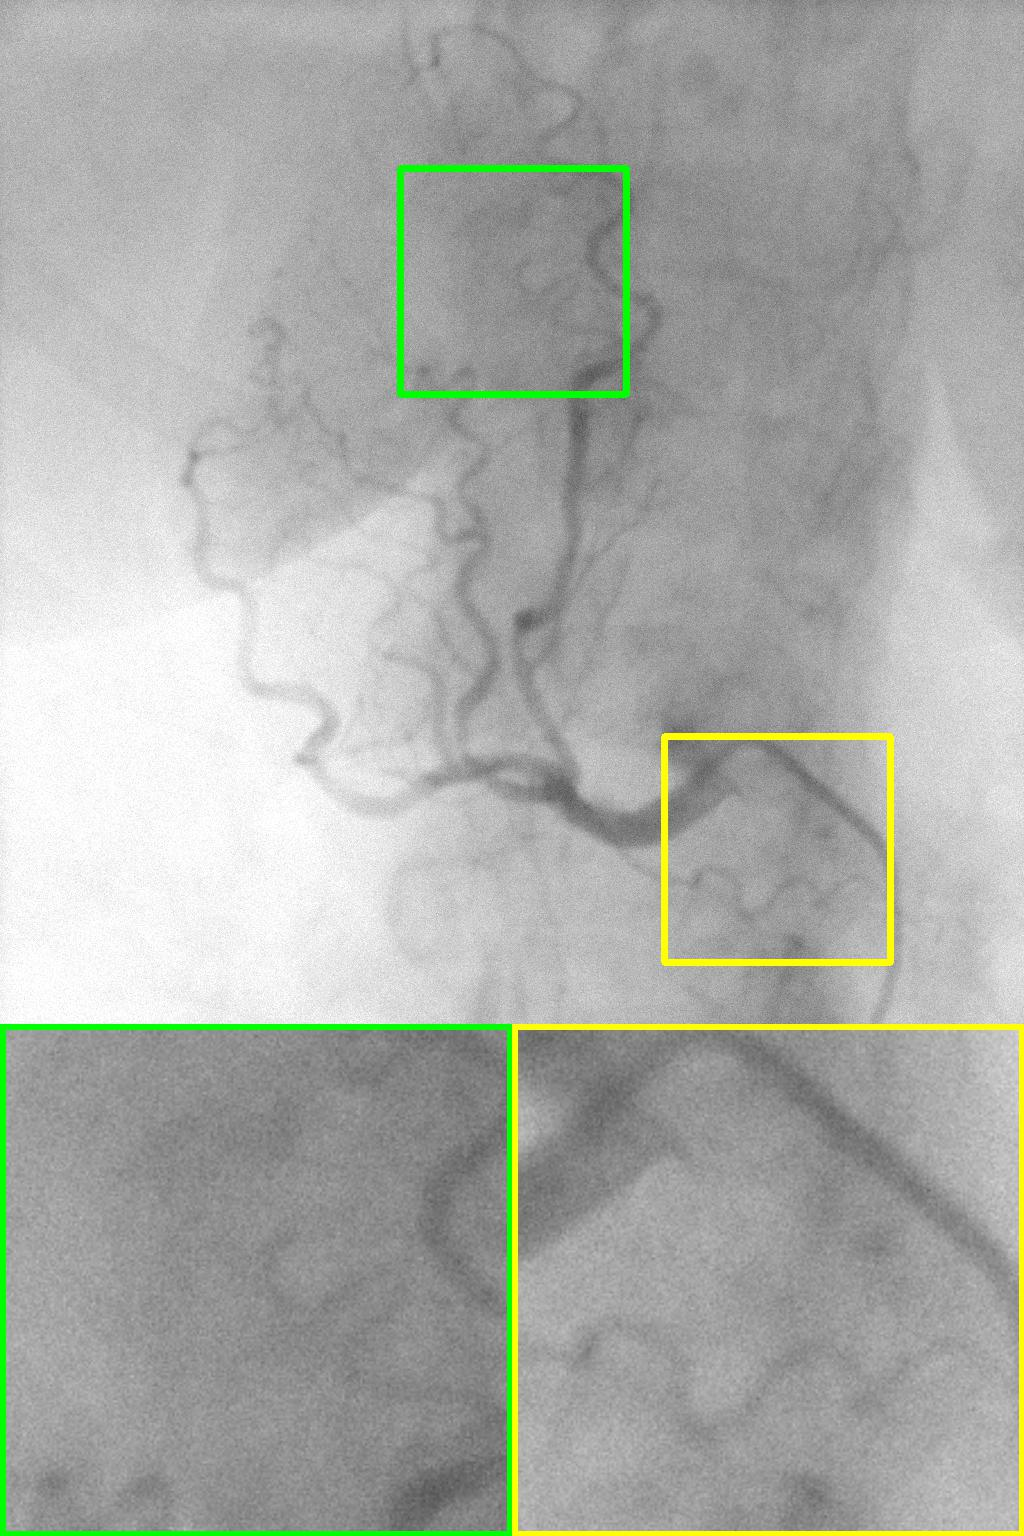} &
    \includegraphics[width=0.083\textwidth]{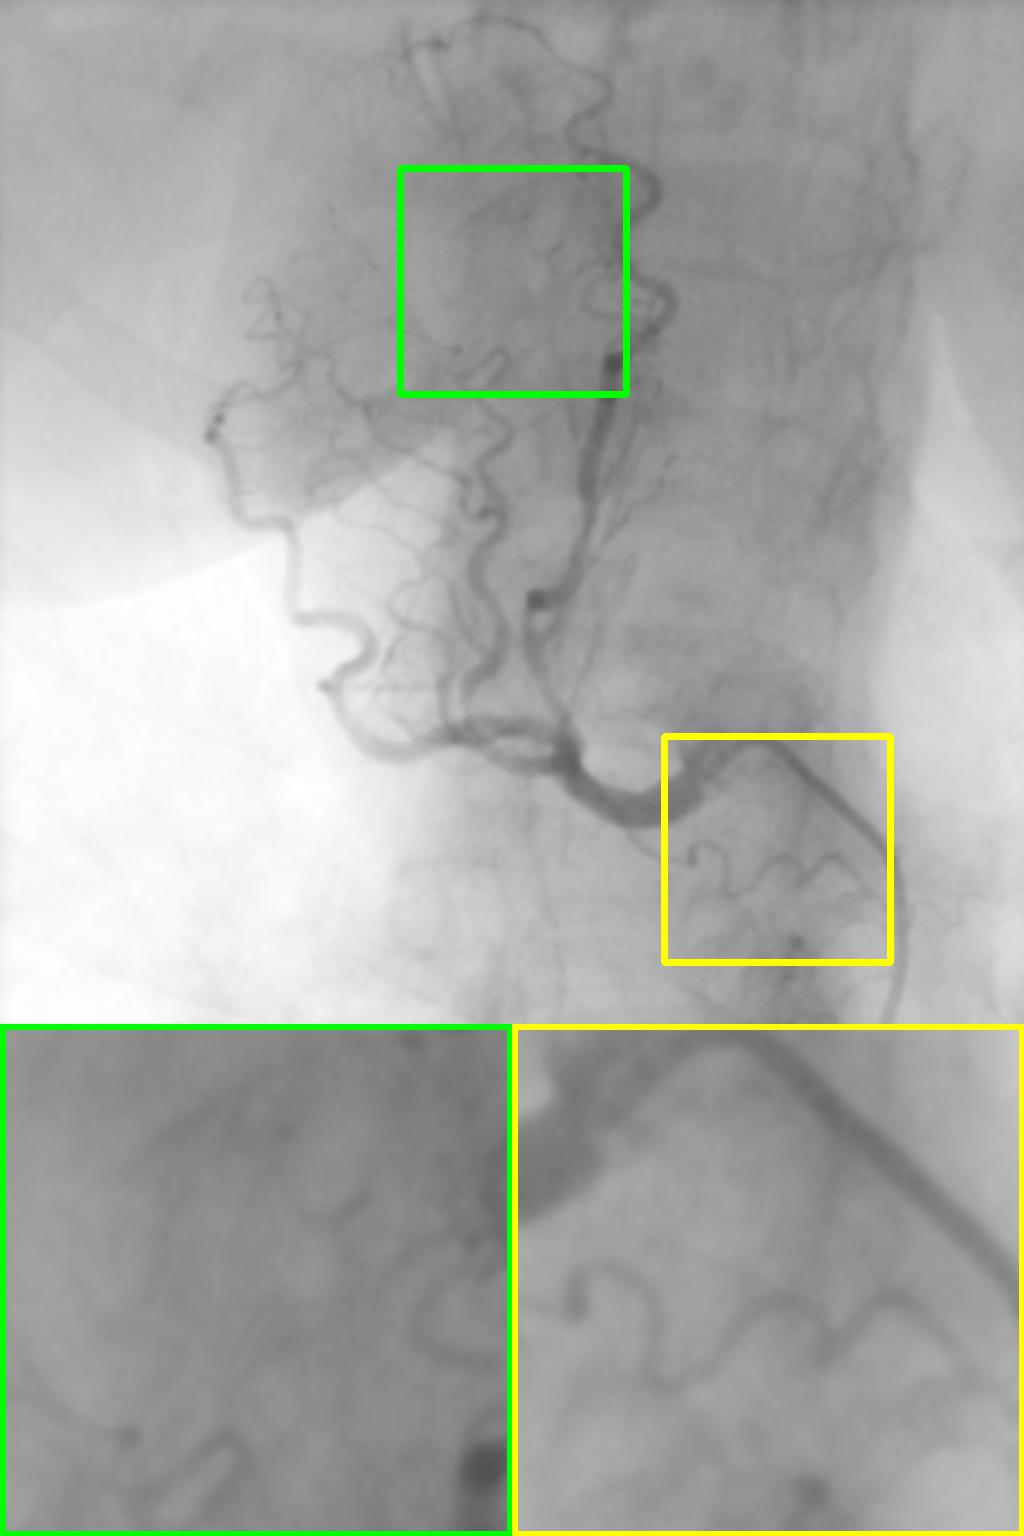} &
    \includegraphics[width=0.083\textwidth]{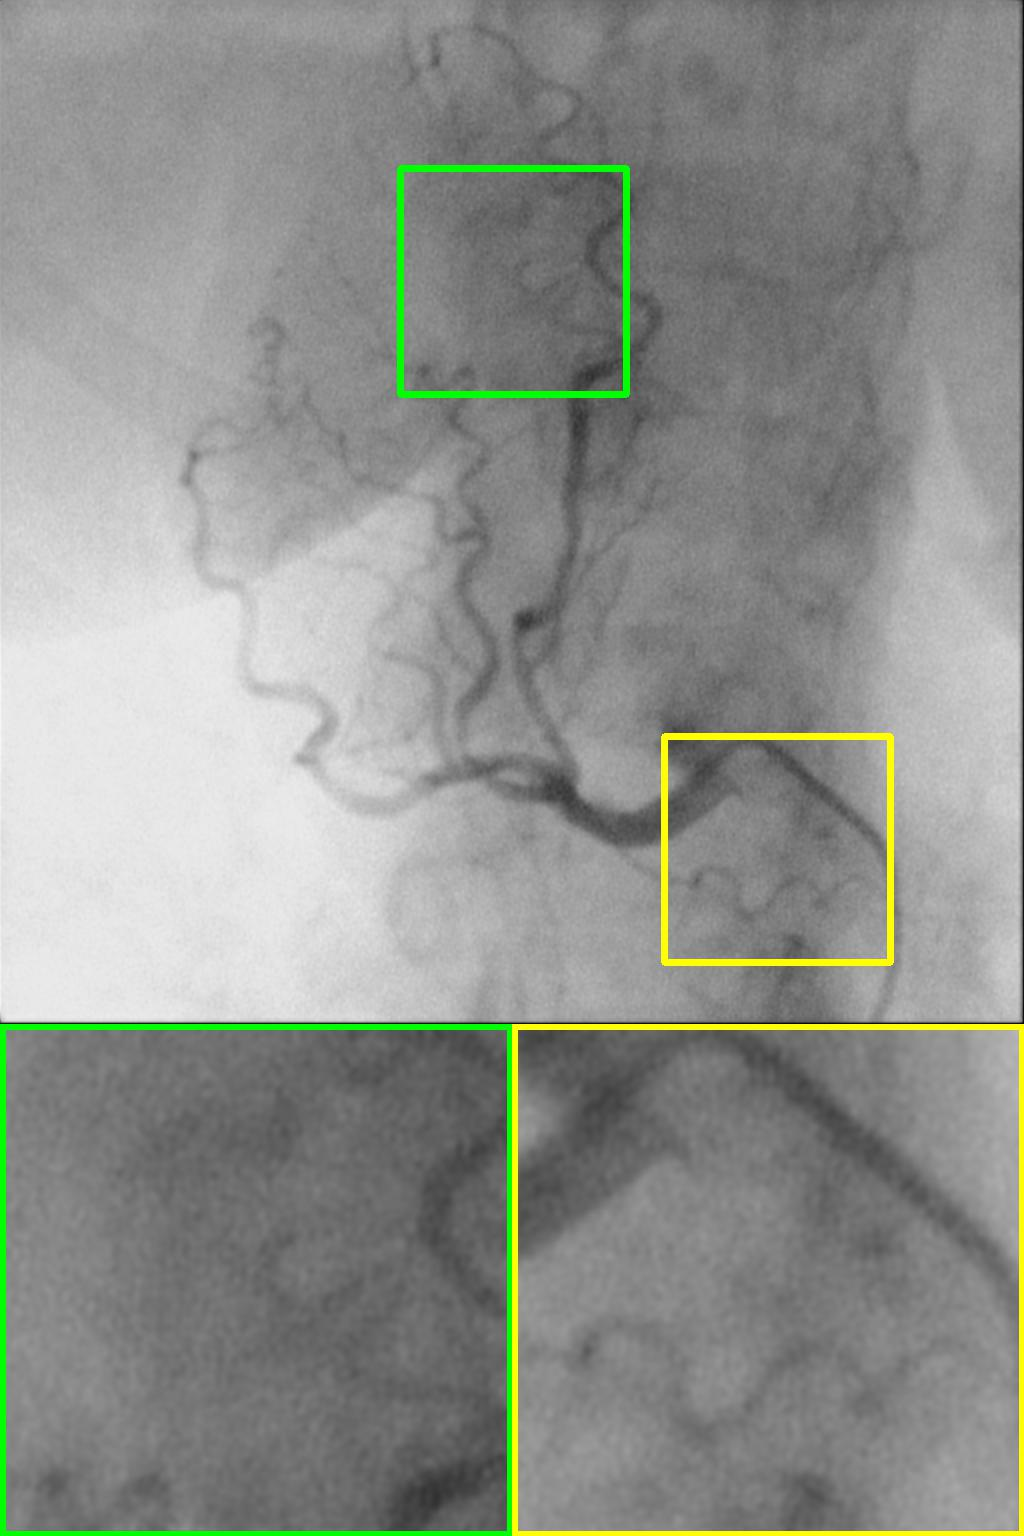}&
    \includegraphics[width=0.083\textwidth]{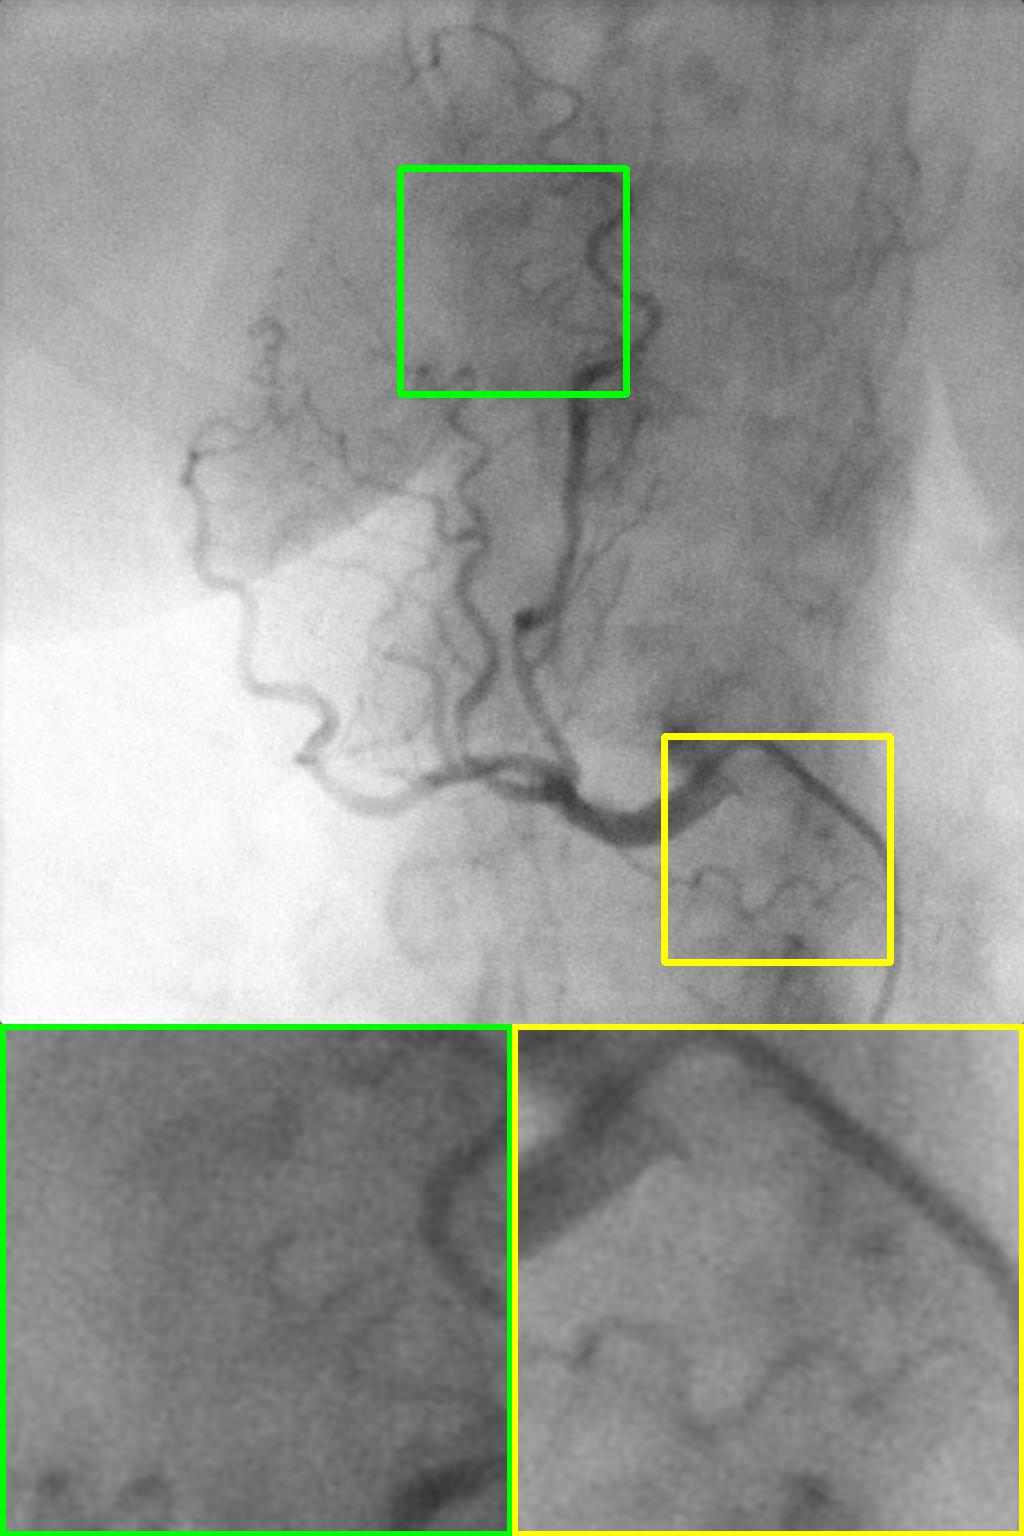}&
    \includegraphics[width=0.083\textwidth]{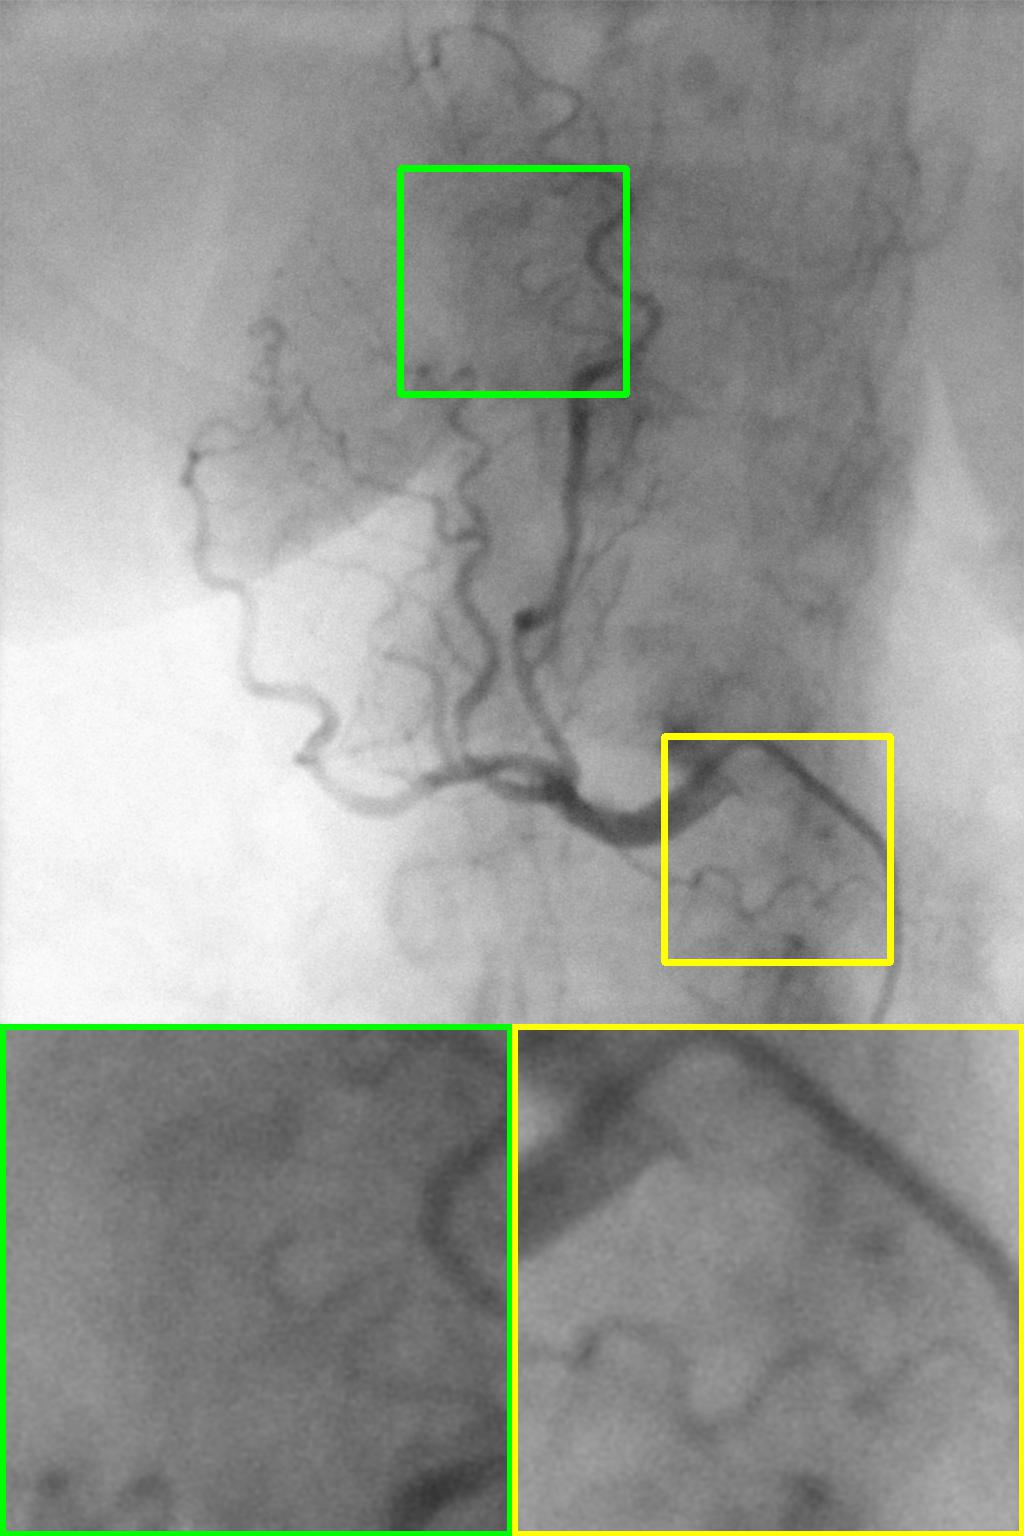}&
    \includegraphics[width=0.083\textwidth]{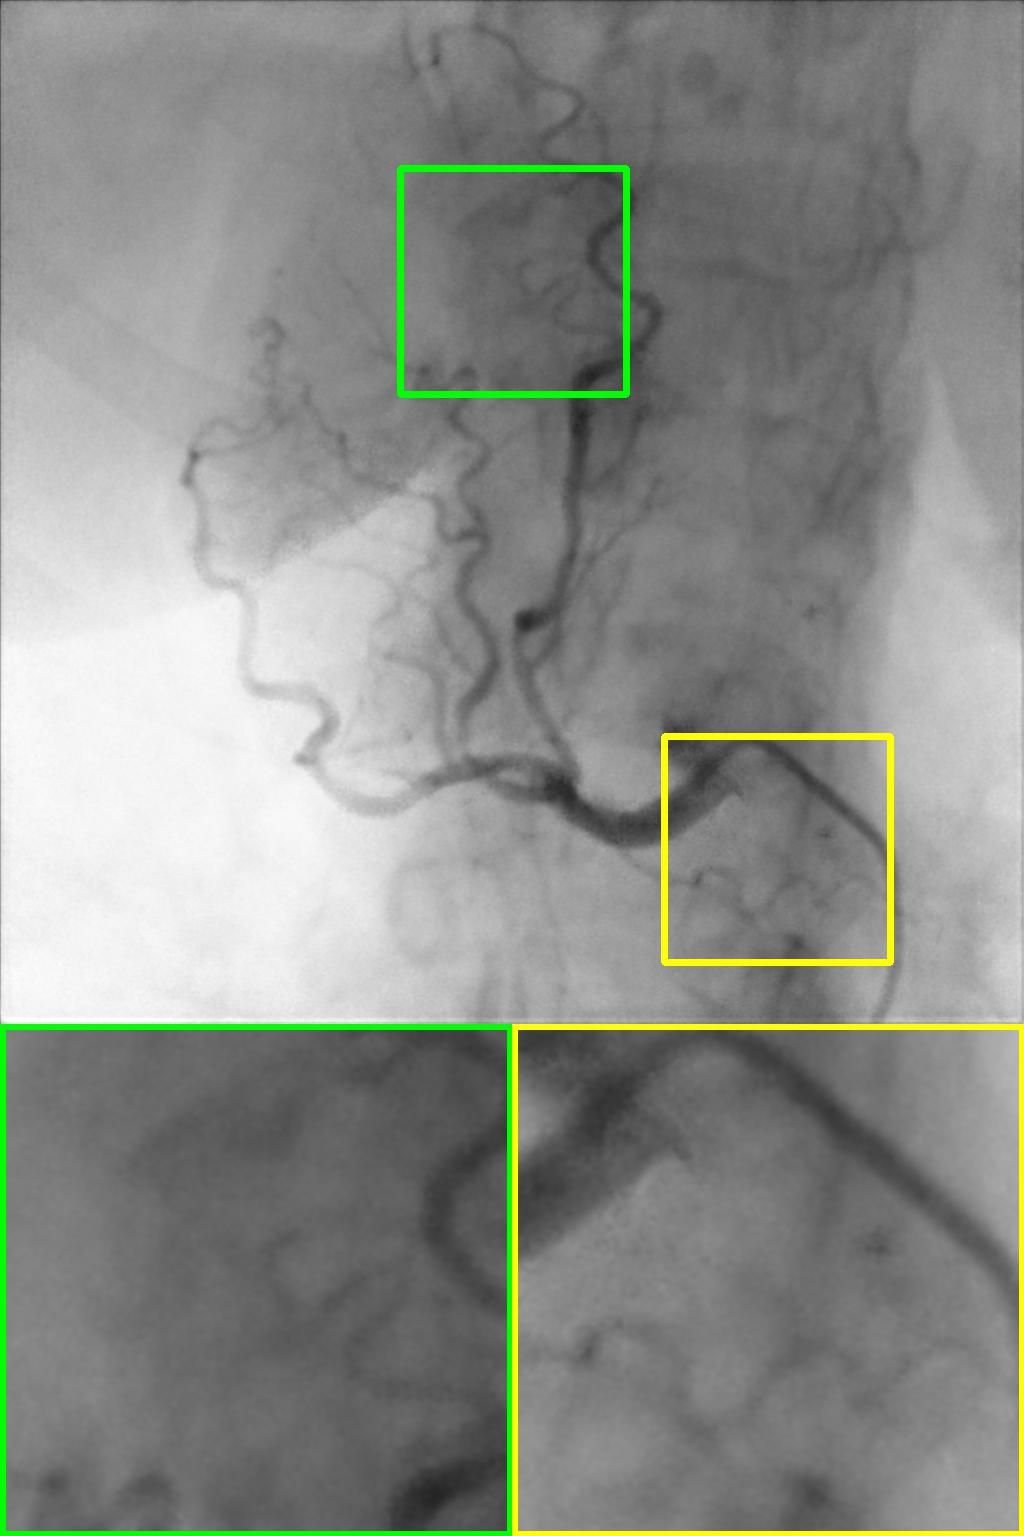}&
    \end{tabular}
}
\caption{Left: Visual comparison of denoising results. They are Gaussian noise with sigma 0.001. }
\label{t2}
\end{figure}
