# Supplementary material for: Stabilize, Decompose, and Denoise: Self-Supervised Fluoroscopy Denoising
Source: arXiv:2208.14022 source file (2022-08-30)
Supplement: Supplementary file 4 [file t3.tex]

% Please add the following required packages to your document preamble:
% \usepackage{multirow}
\begin{table}[]
\centering
\caption{Denoising  result  of  video  7  proccessed}
\begin{tabular}{|c|c|c|c|}
\hline
                          &      & Ours          & Self2self          \\ \hline
\multirow{3}{*}{Gaussian} & 0.01 & "7\_0.01.mp4" & "7\_0.01\_s2s.mp4" \\ \cline{2-4} 
                          & 0.03 & "7\_0.03.mp4" & "7\_0.03\_s2s.mp4" \\ \cline{2-4} 
                          & 0.05 & "7\_0.05.mp4" & "7\_0.05\_s2s.mp4" \\ \hline
\end{tabular}
\label{t3}
\end{table}
